# Supplementary material for: iToF2dToF: A Robust and Flexible Representation for Data-Driven Time-of-Flight Imaging
Source: arXiv:2103.07087 source file (2021-12-21)
Supplement: Supplementary file 1 [file freq_analysis.tex]

\label{sec:freq}
% \subsection{}
% \textbf{What is the minimum bandwidth needed to resolve MPI?}
% In this section, we empirically demonstrate that one only need to sample frequencies up to around 300MHz to largely mitigate MPI in indoor scenes. We study indoor scenes because I-ToF cameras are mainly used indoors. Then we introduce a data-driven framework that interpolates and extrapolates a few I-ToF frequency samples up to 300MHz, effectively mitigating MPI. Finally, we combine this framework with a simple and robust depth estimation algorithm.
% \begin{figure*}[t]
% \label{fig:localerrorsanalysis}
% \centering
% \includegraphics[width=\textwidth]{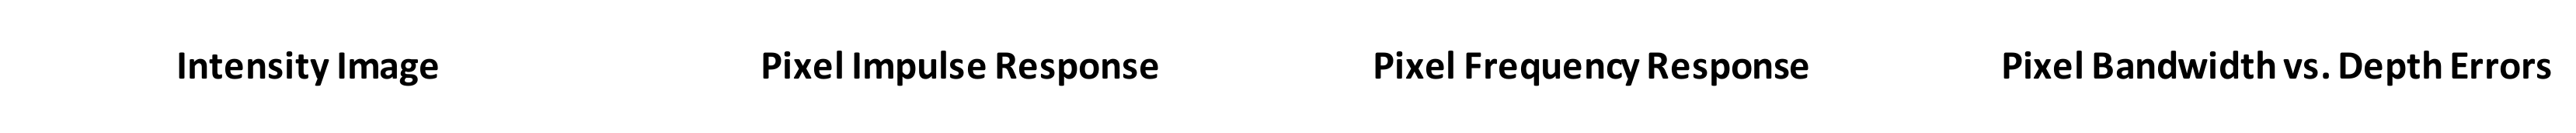}
% \includegraphics[width=\textwidth]{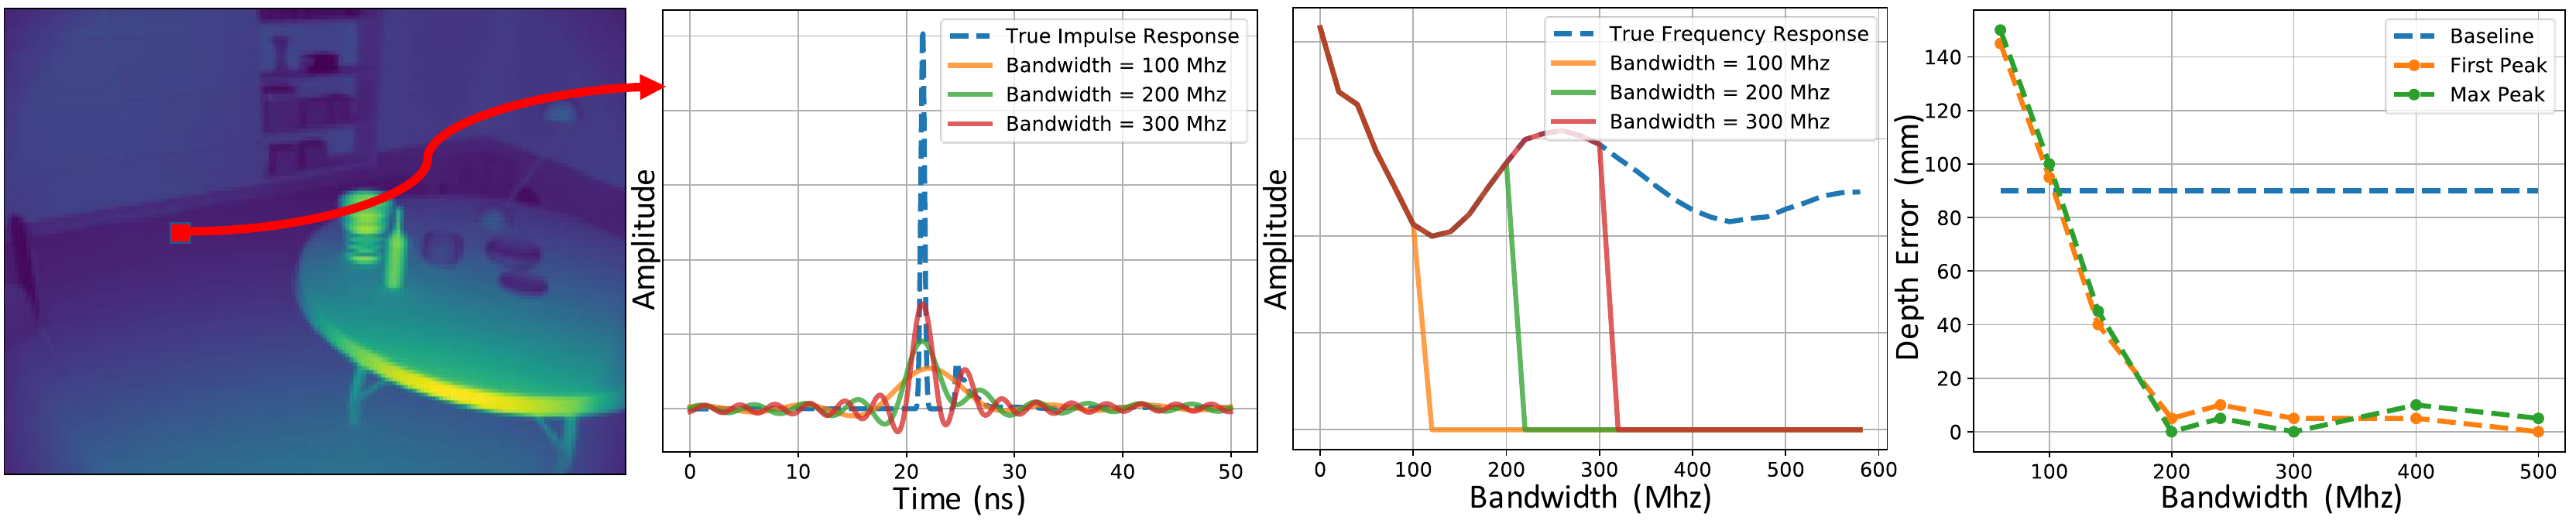}
% \caption{\textbf{Bandwidth vs. Local MPI Depth Errors}.}
% \end{figure*}

% \rnote{Maybe this section can just go in the supplement. And just write a sentence or two about this. }
% We find that we can get close to minimizing MPI in most indoor scenes by capturing up to 300MHz.

% \begin{figure}[t]
% \label{fig:globalerrorsanalysis}
% \centering
% \includegraphics[width=0.5\textwidth]{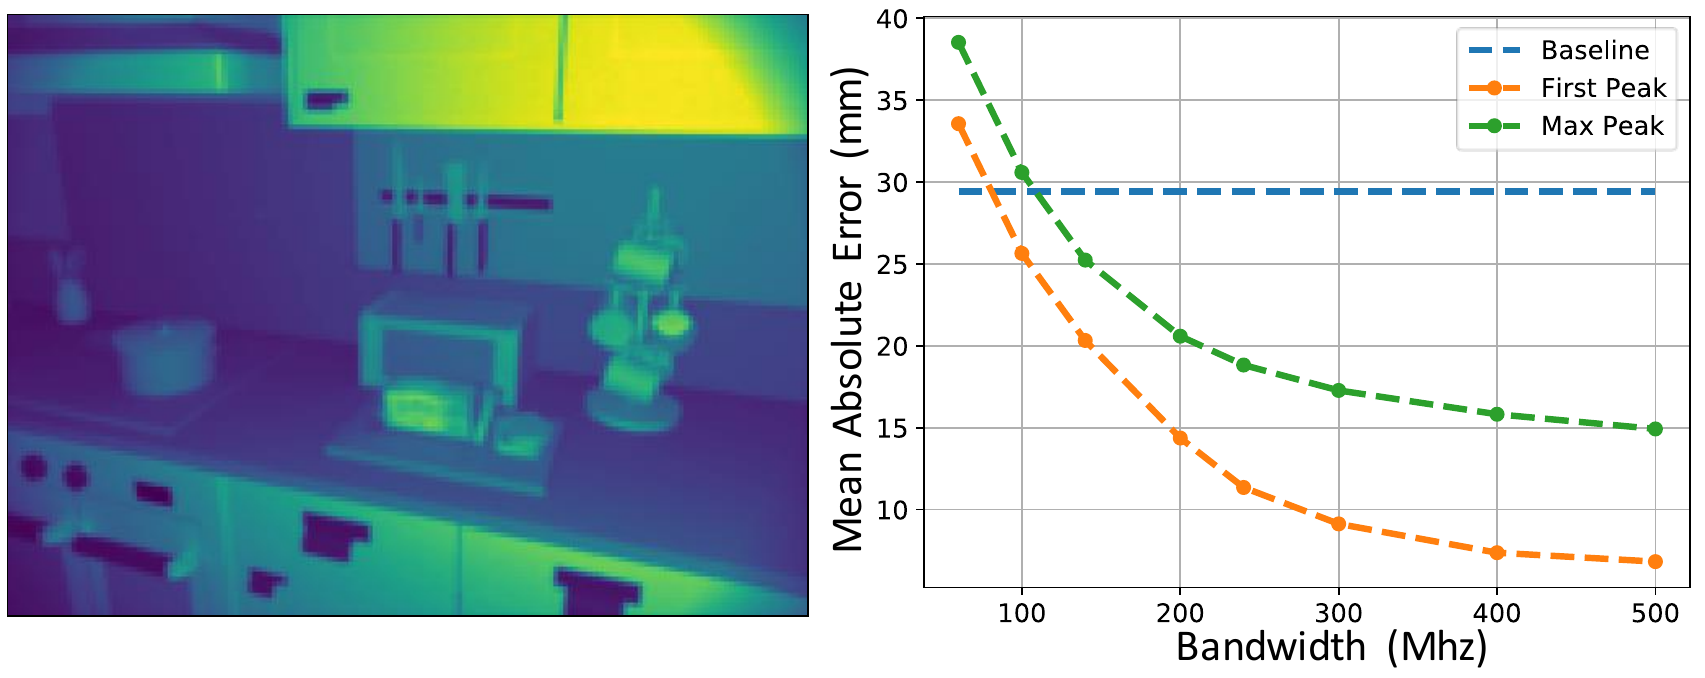}
% \caption{\textbf{Bandwidth vs. Global MPI Depth Errors}.}
% \end{figure}

% \begin{figure}[t]
% \label{fig:fit}
% \centering
%   \includegraphics[width=0.45\textwidth]{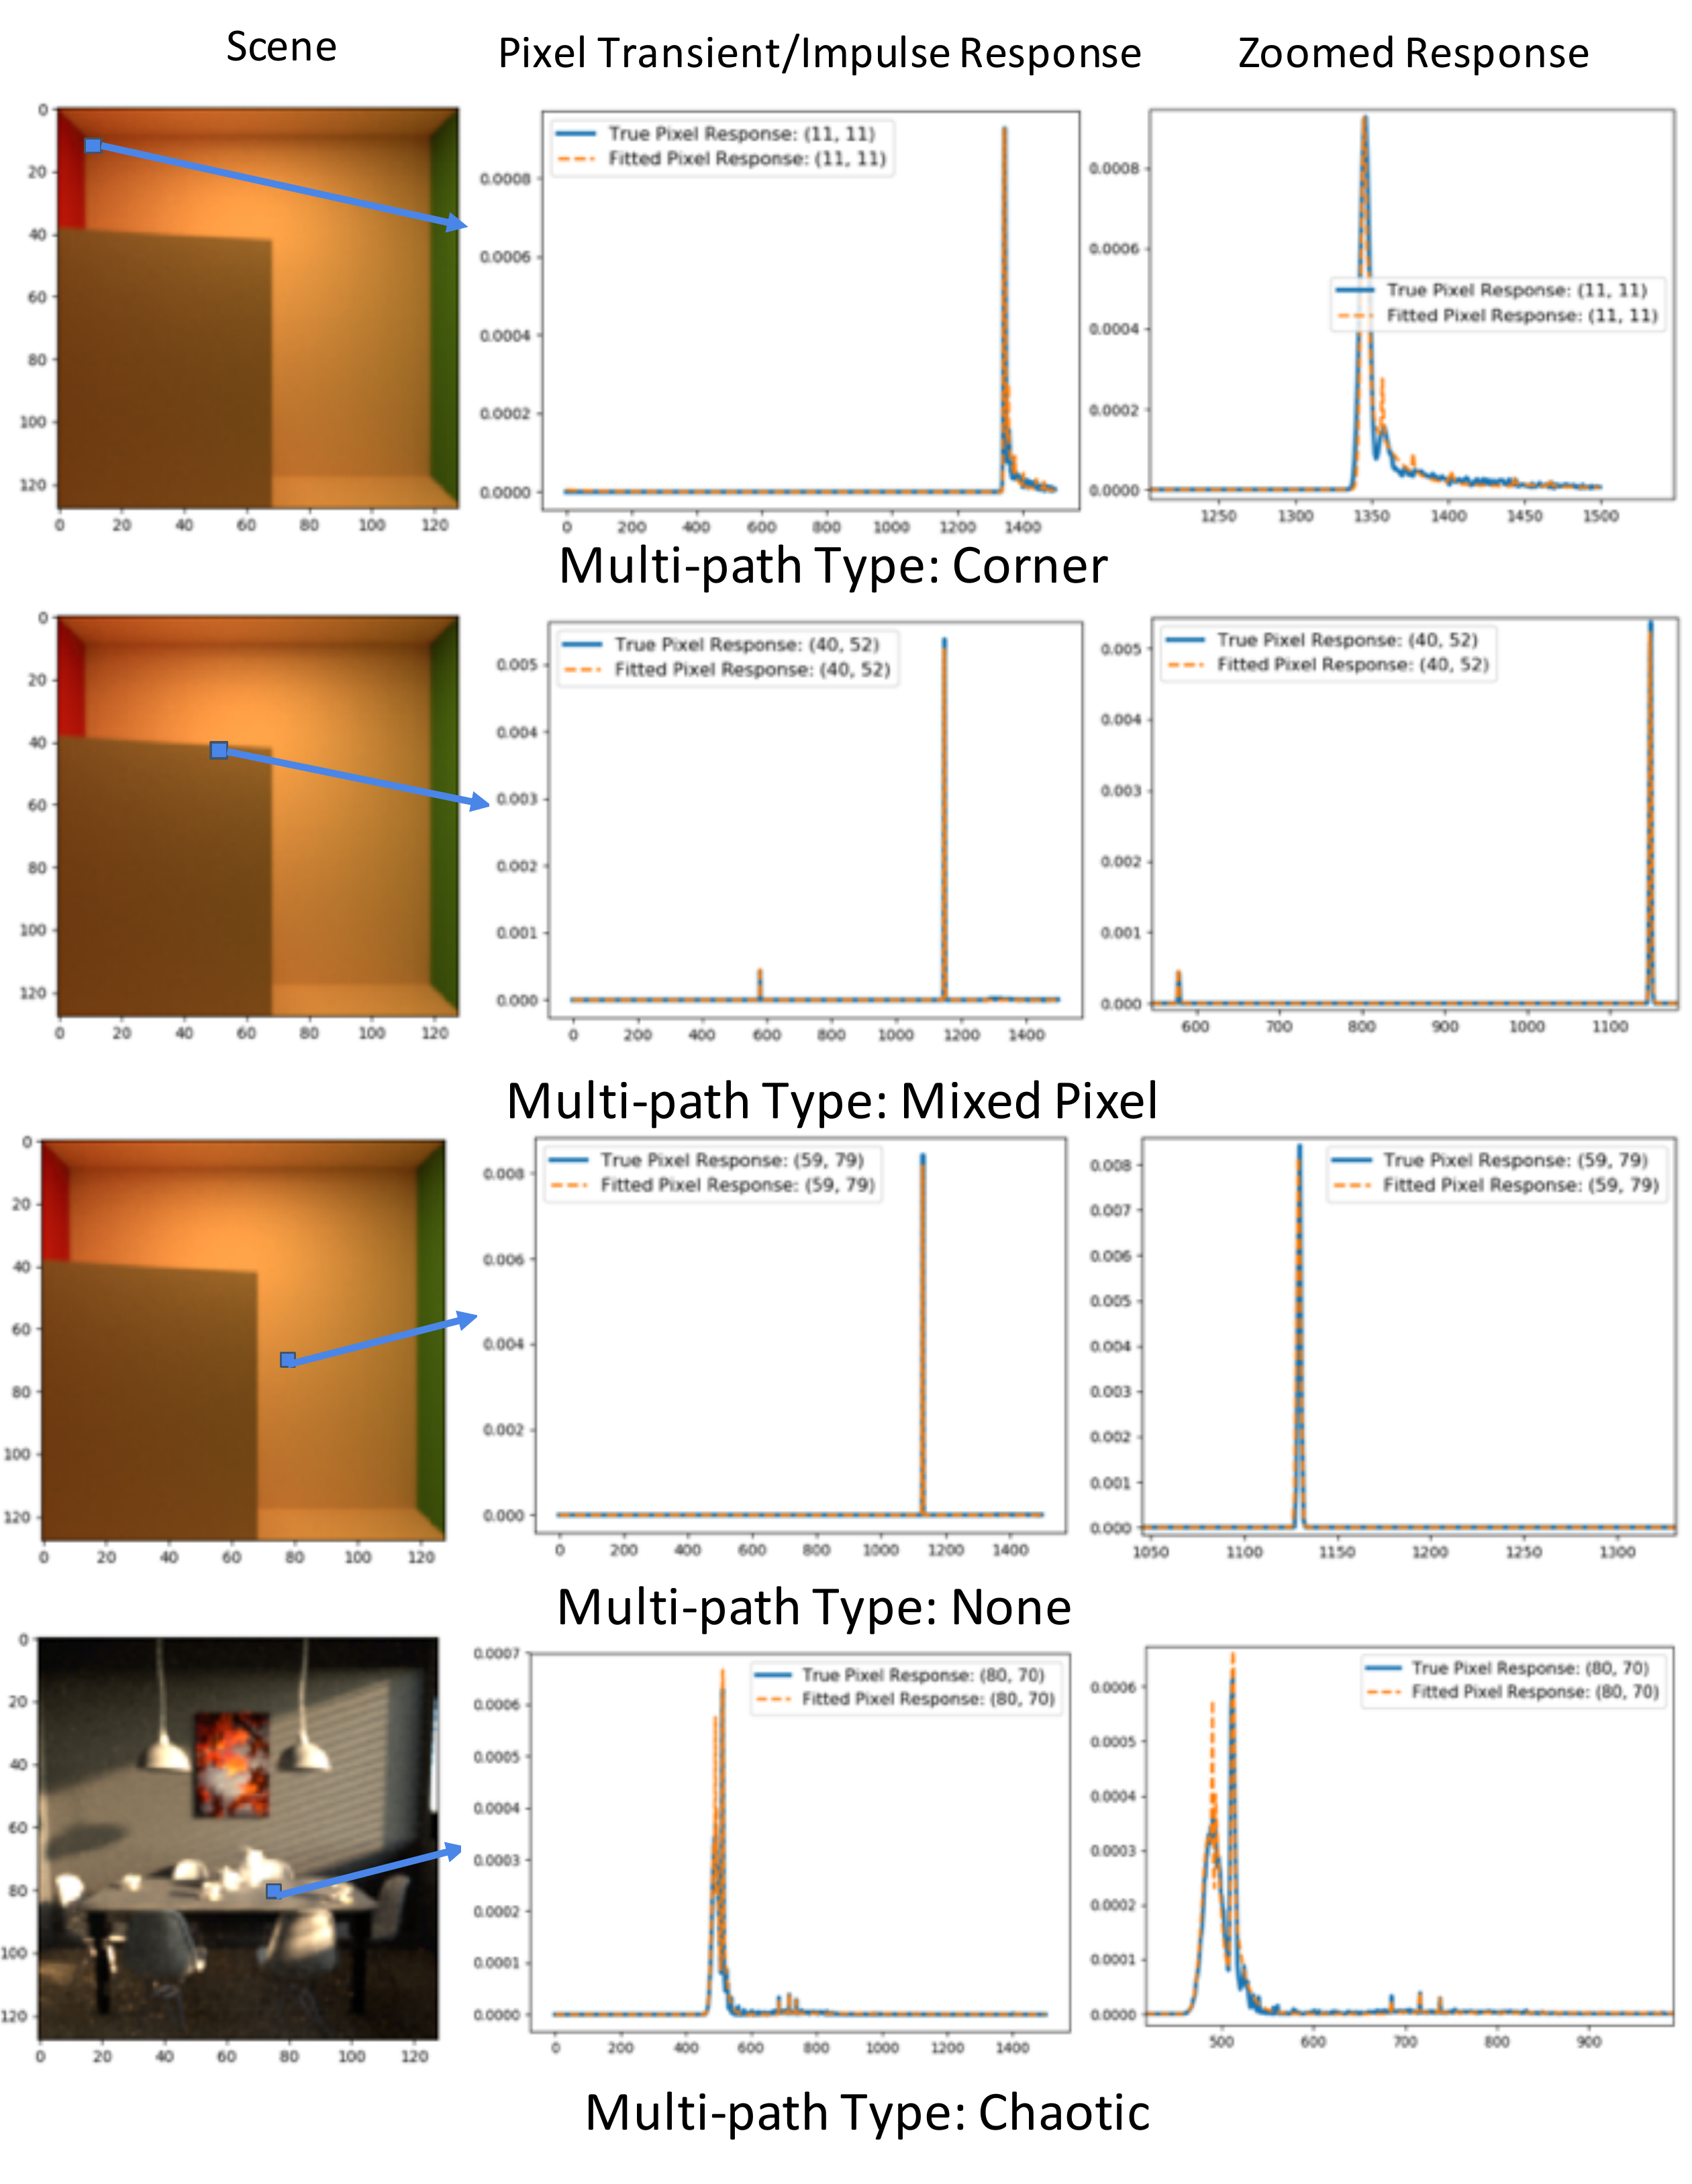}
% \caption{Example two-column figure.}
% \end{figure}
