# Supplementary material for: iToF2dToF: A Robust and Flexible Representation for Data-Driven Time-of-Flight Imaging
Source: arXiv:2103.07087 source file (2021-12-21)
Supplement: Supplementary file 2 [file supplement-5_experimental_setup.tex]

\clearpage
\section{Experimental Setup}
\label{sec:supplement-4_experimental_setup}

\subsection{Data Acquisition}

\noindent \textbf{iToF Module:} The iToF module we use for the real experiments is the Sony IMX516 iToF sensor. The sensor has VGA resolution (480x640 pixels) and a horizontal field of view of ~60 degrees. We are able to control the exposure time from 0.1ms up to 1ms. The module has a light source whose average illumination power is 1W. The IMX516 is configured and calibrated to take measurements at 20MHz and 100MHz by the manufacturer. We are able to access the raw iToF measurements for these two frequencies. Unfortunately, we are not able to configure or calibrate additional frequencies due to the unavailability of low-level access of the module.  

\medskip

\noindent \textbf{Collected Data and Acquisition Settings: }We acquire a variety of scenes for the qualitative and quantitative evaluation of our models. For all quantitative results, for a given exposure time, we obtain denoised ground truth images by averaging 100 raw ToF frames. The following are the scenes we acquired and the data acquisition settings used:

\begin{itemize}
    \item \textbf{Flat Wall Data}
    \item \textbf{MPI Scenes}
    \item \textbf{Cross-talk Scene}
    \item \textbf{Specular MPI Scene}
\end{itemize}

\subsection{Partial Ground Truth for Real-world Scene}
