# Supplementary material for: iToF2dToF: A Robust and Flexible Representation for Data-Driven Time-of-Flight Imaging
Source: arXiv:2103.07087 source file (2021-12-21)
Supplement: Supplementary file 4 [file supplement-1_wall_depth_stats.tex]

\clearpage
\section{Robustness to Noise in Real Data}
\label{sec:supplement-1_robustness}

Figure \ref{fig:supplement_noise_var} shows the variance of depth reconstructions.

\begin{figure}[H]
\centering
    \includegraphics[width=0.99\textwidth]{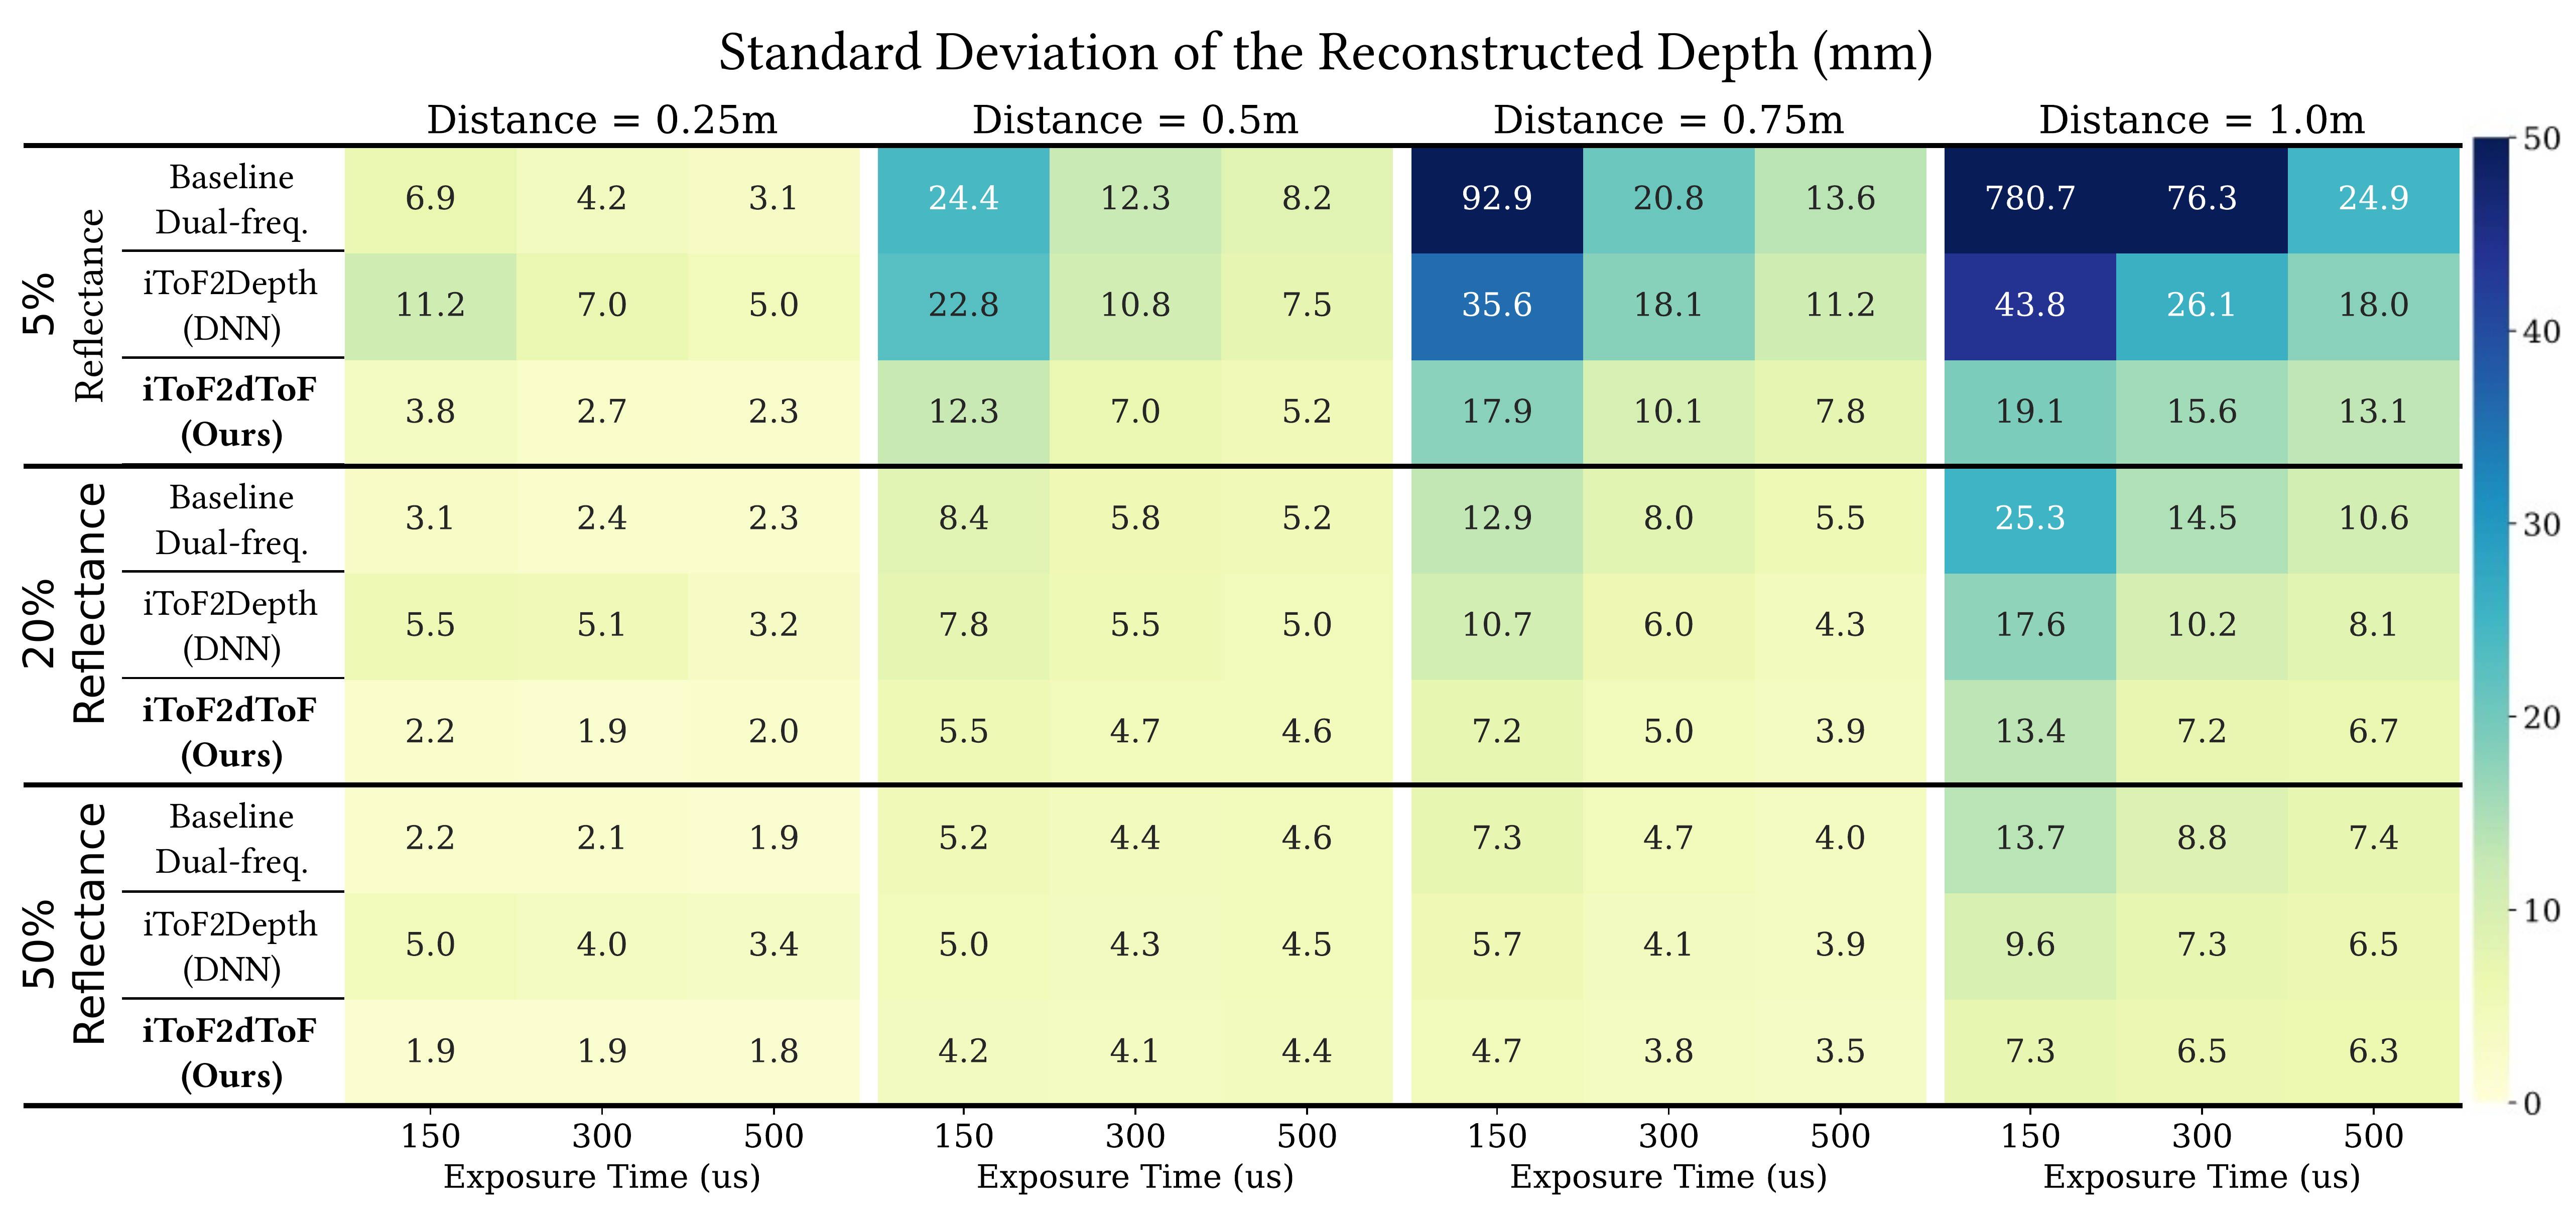}
    \includegraphics[width=0.99\textwidth]{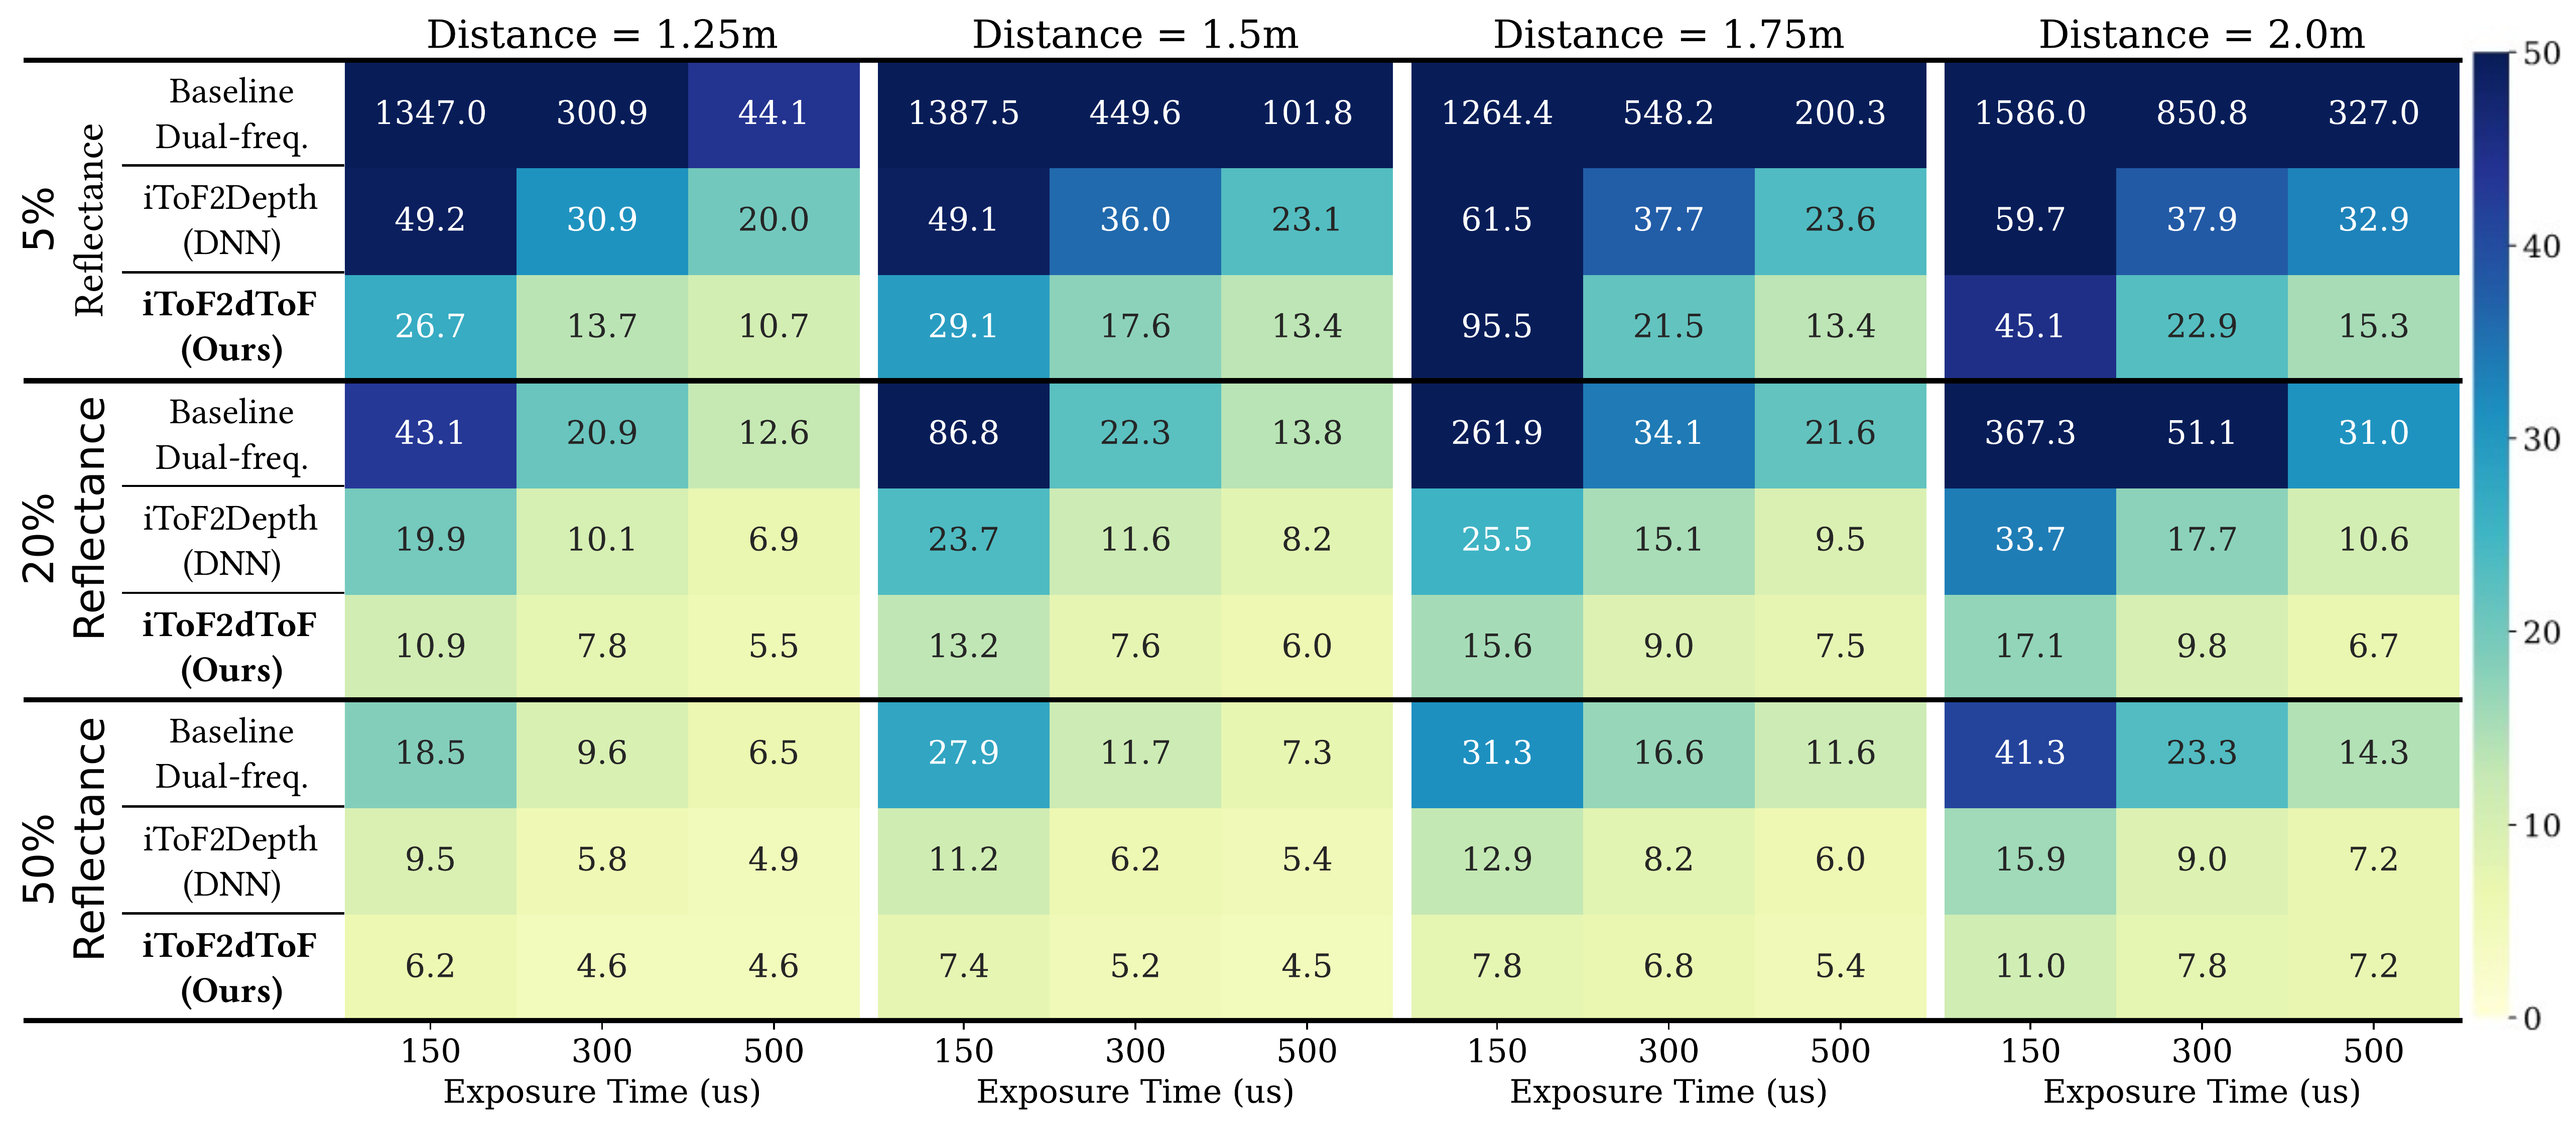}
\caption{\textbf{Wall Depths Standard Deviation}.}
\label{fig:supplement_noise_var}
\end{figure}

\begin{figure}[H]
\centering
    \includegraphics[width=0.48\textwidth]{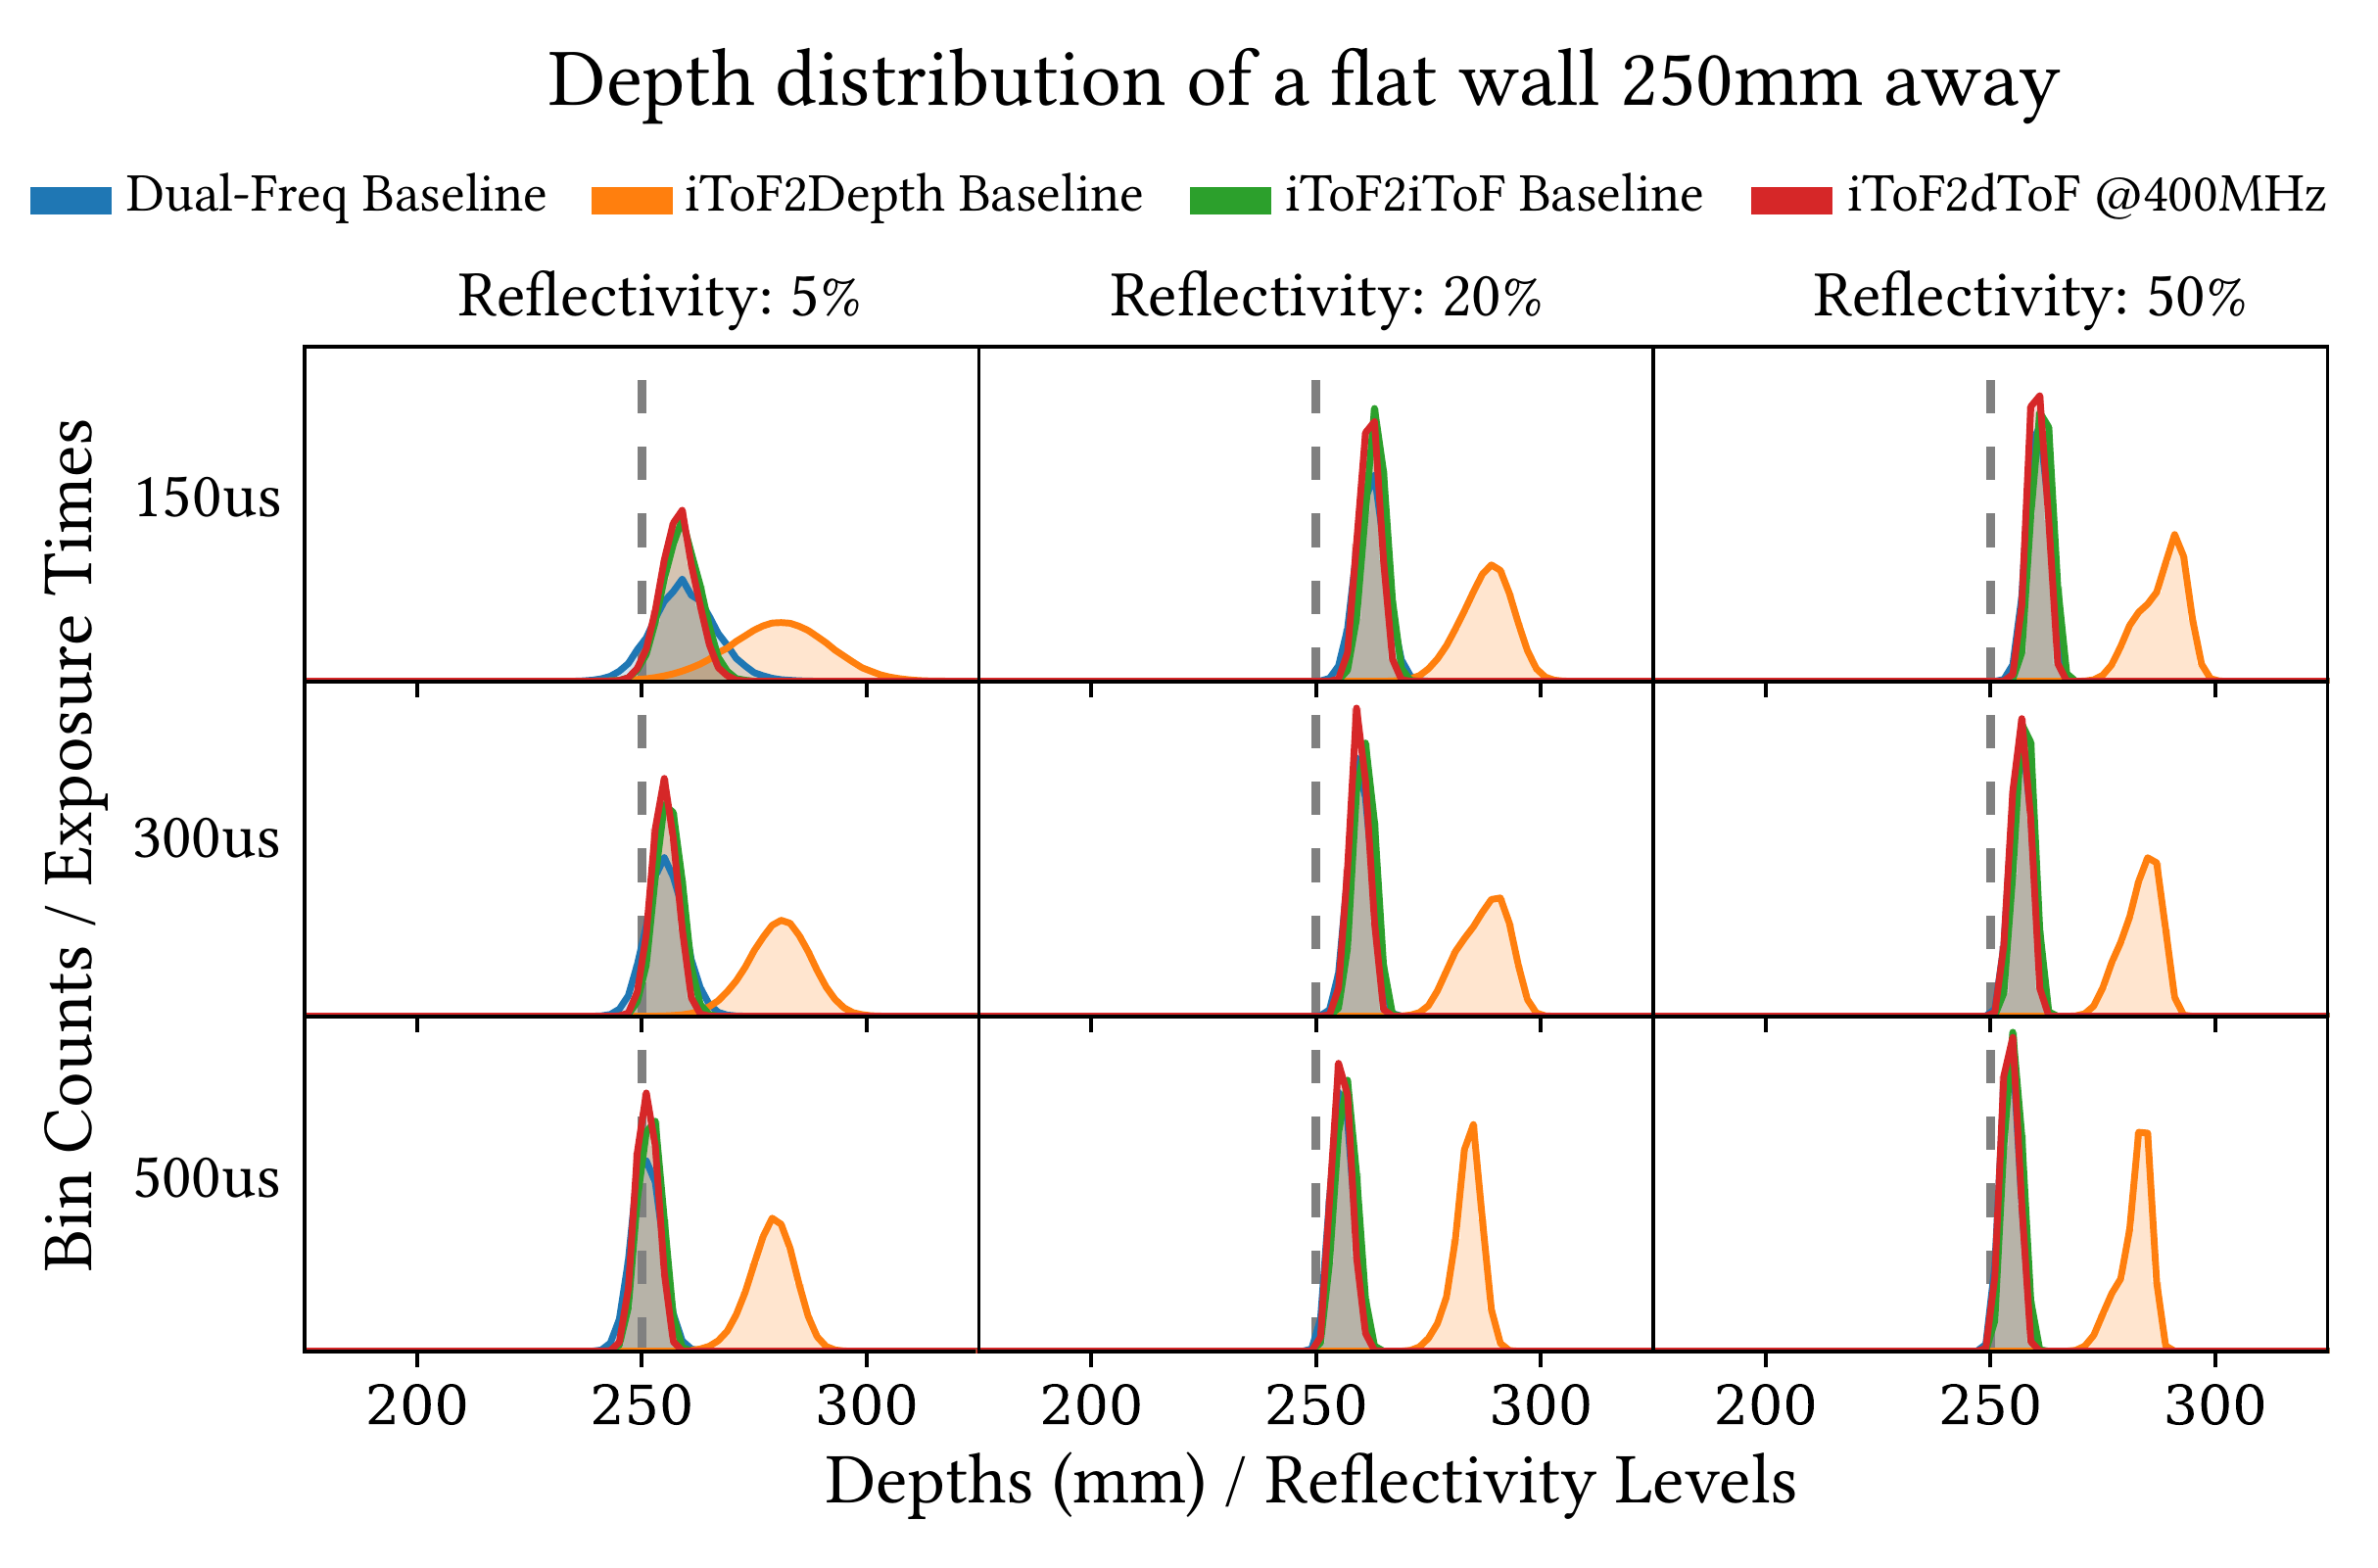}
    \includegraphics[width=0.48\textwidth]{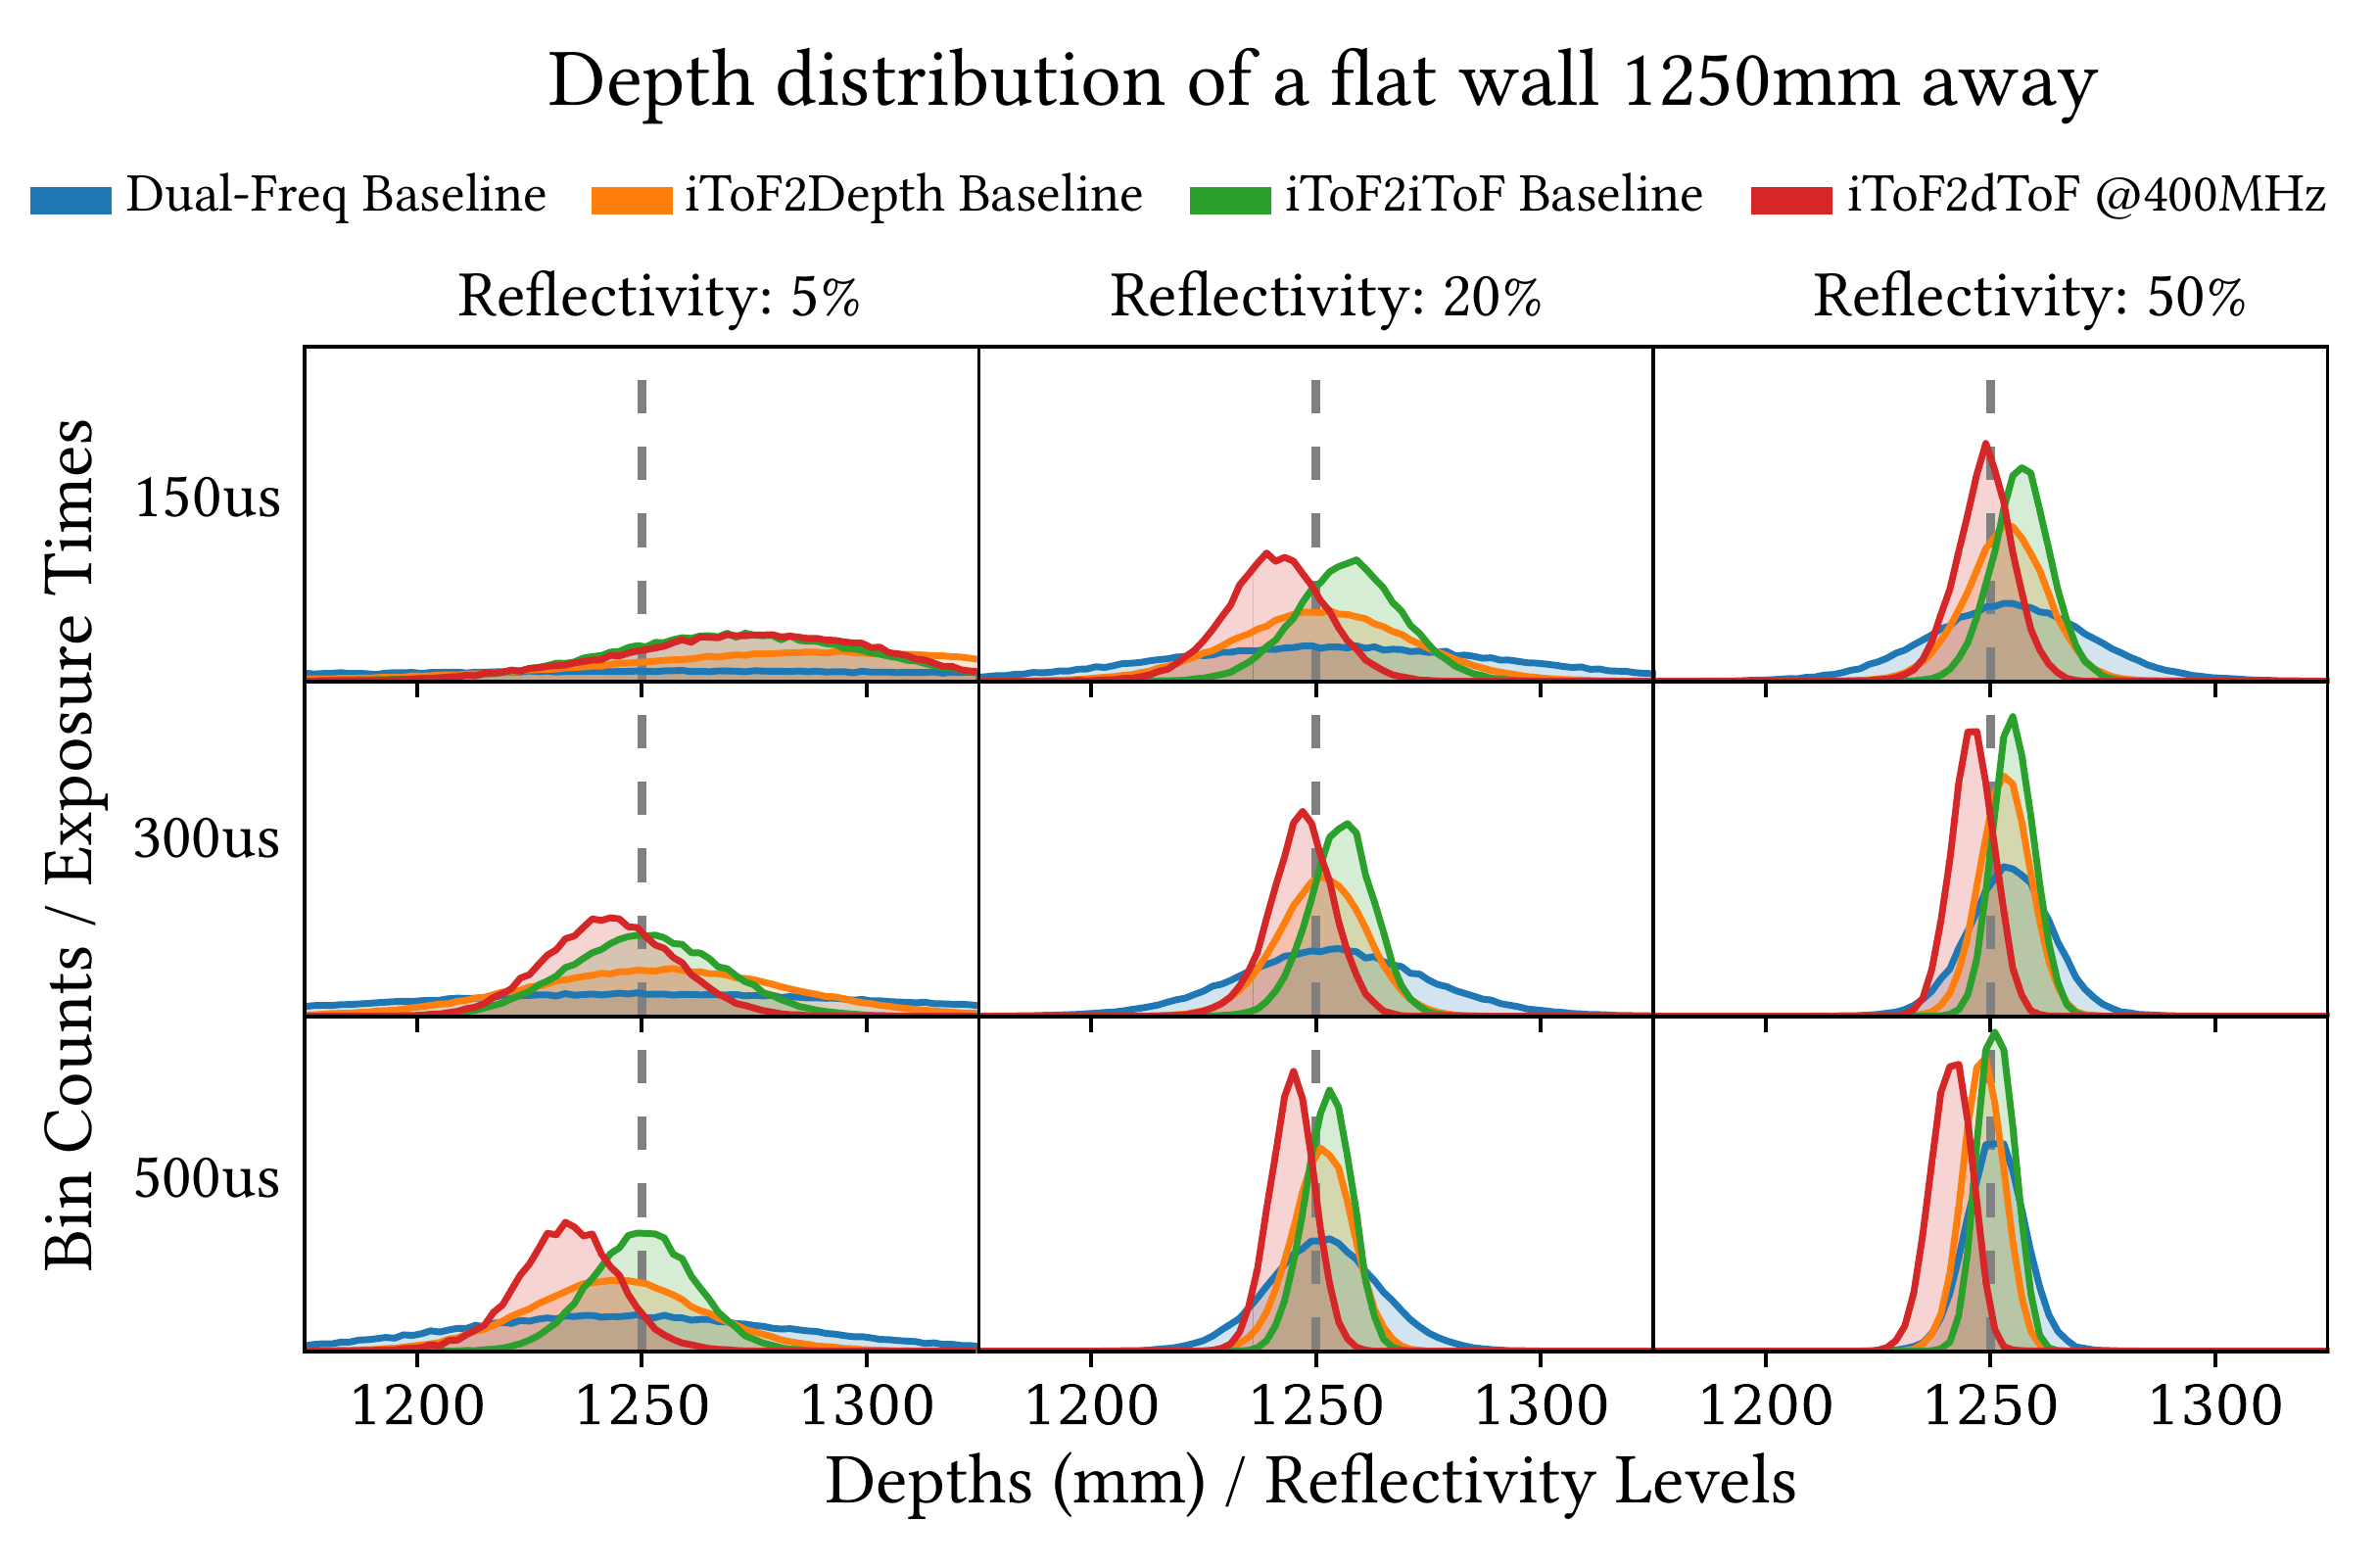}
    \includegraphics[width=0.48\textwidth]{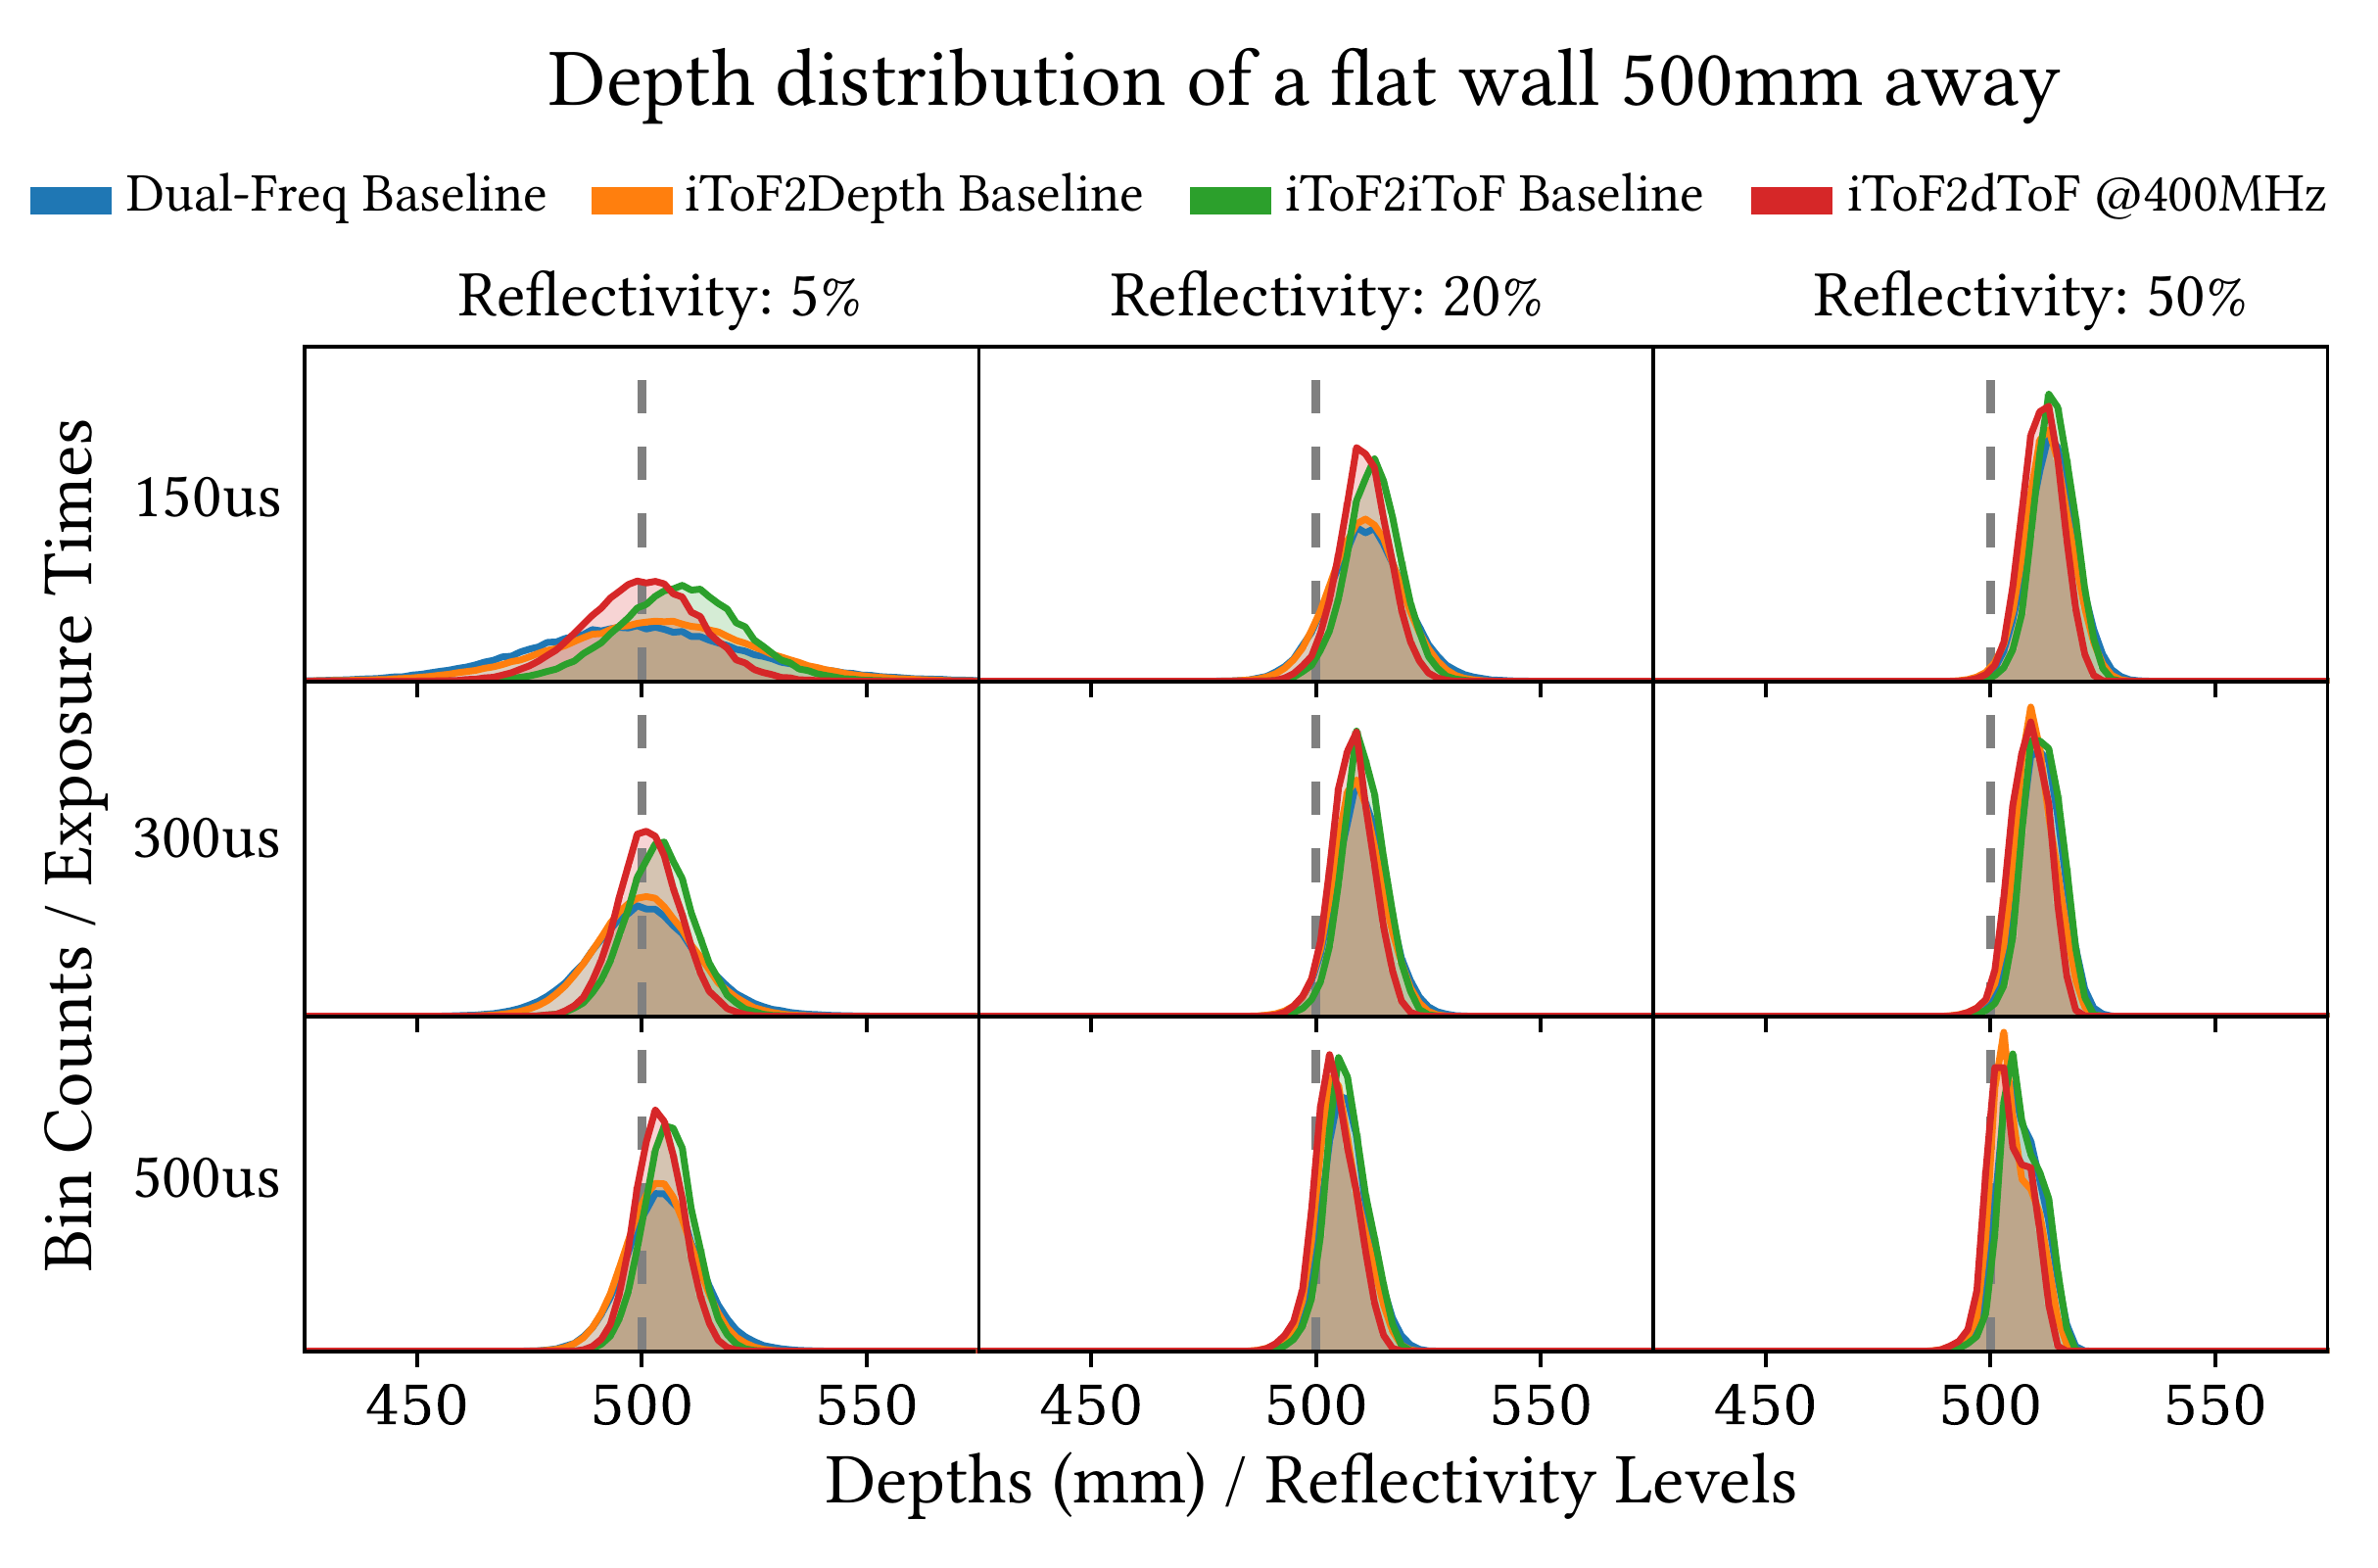}
    \includegraphics[width=0.48\textwidth]{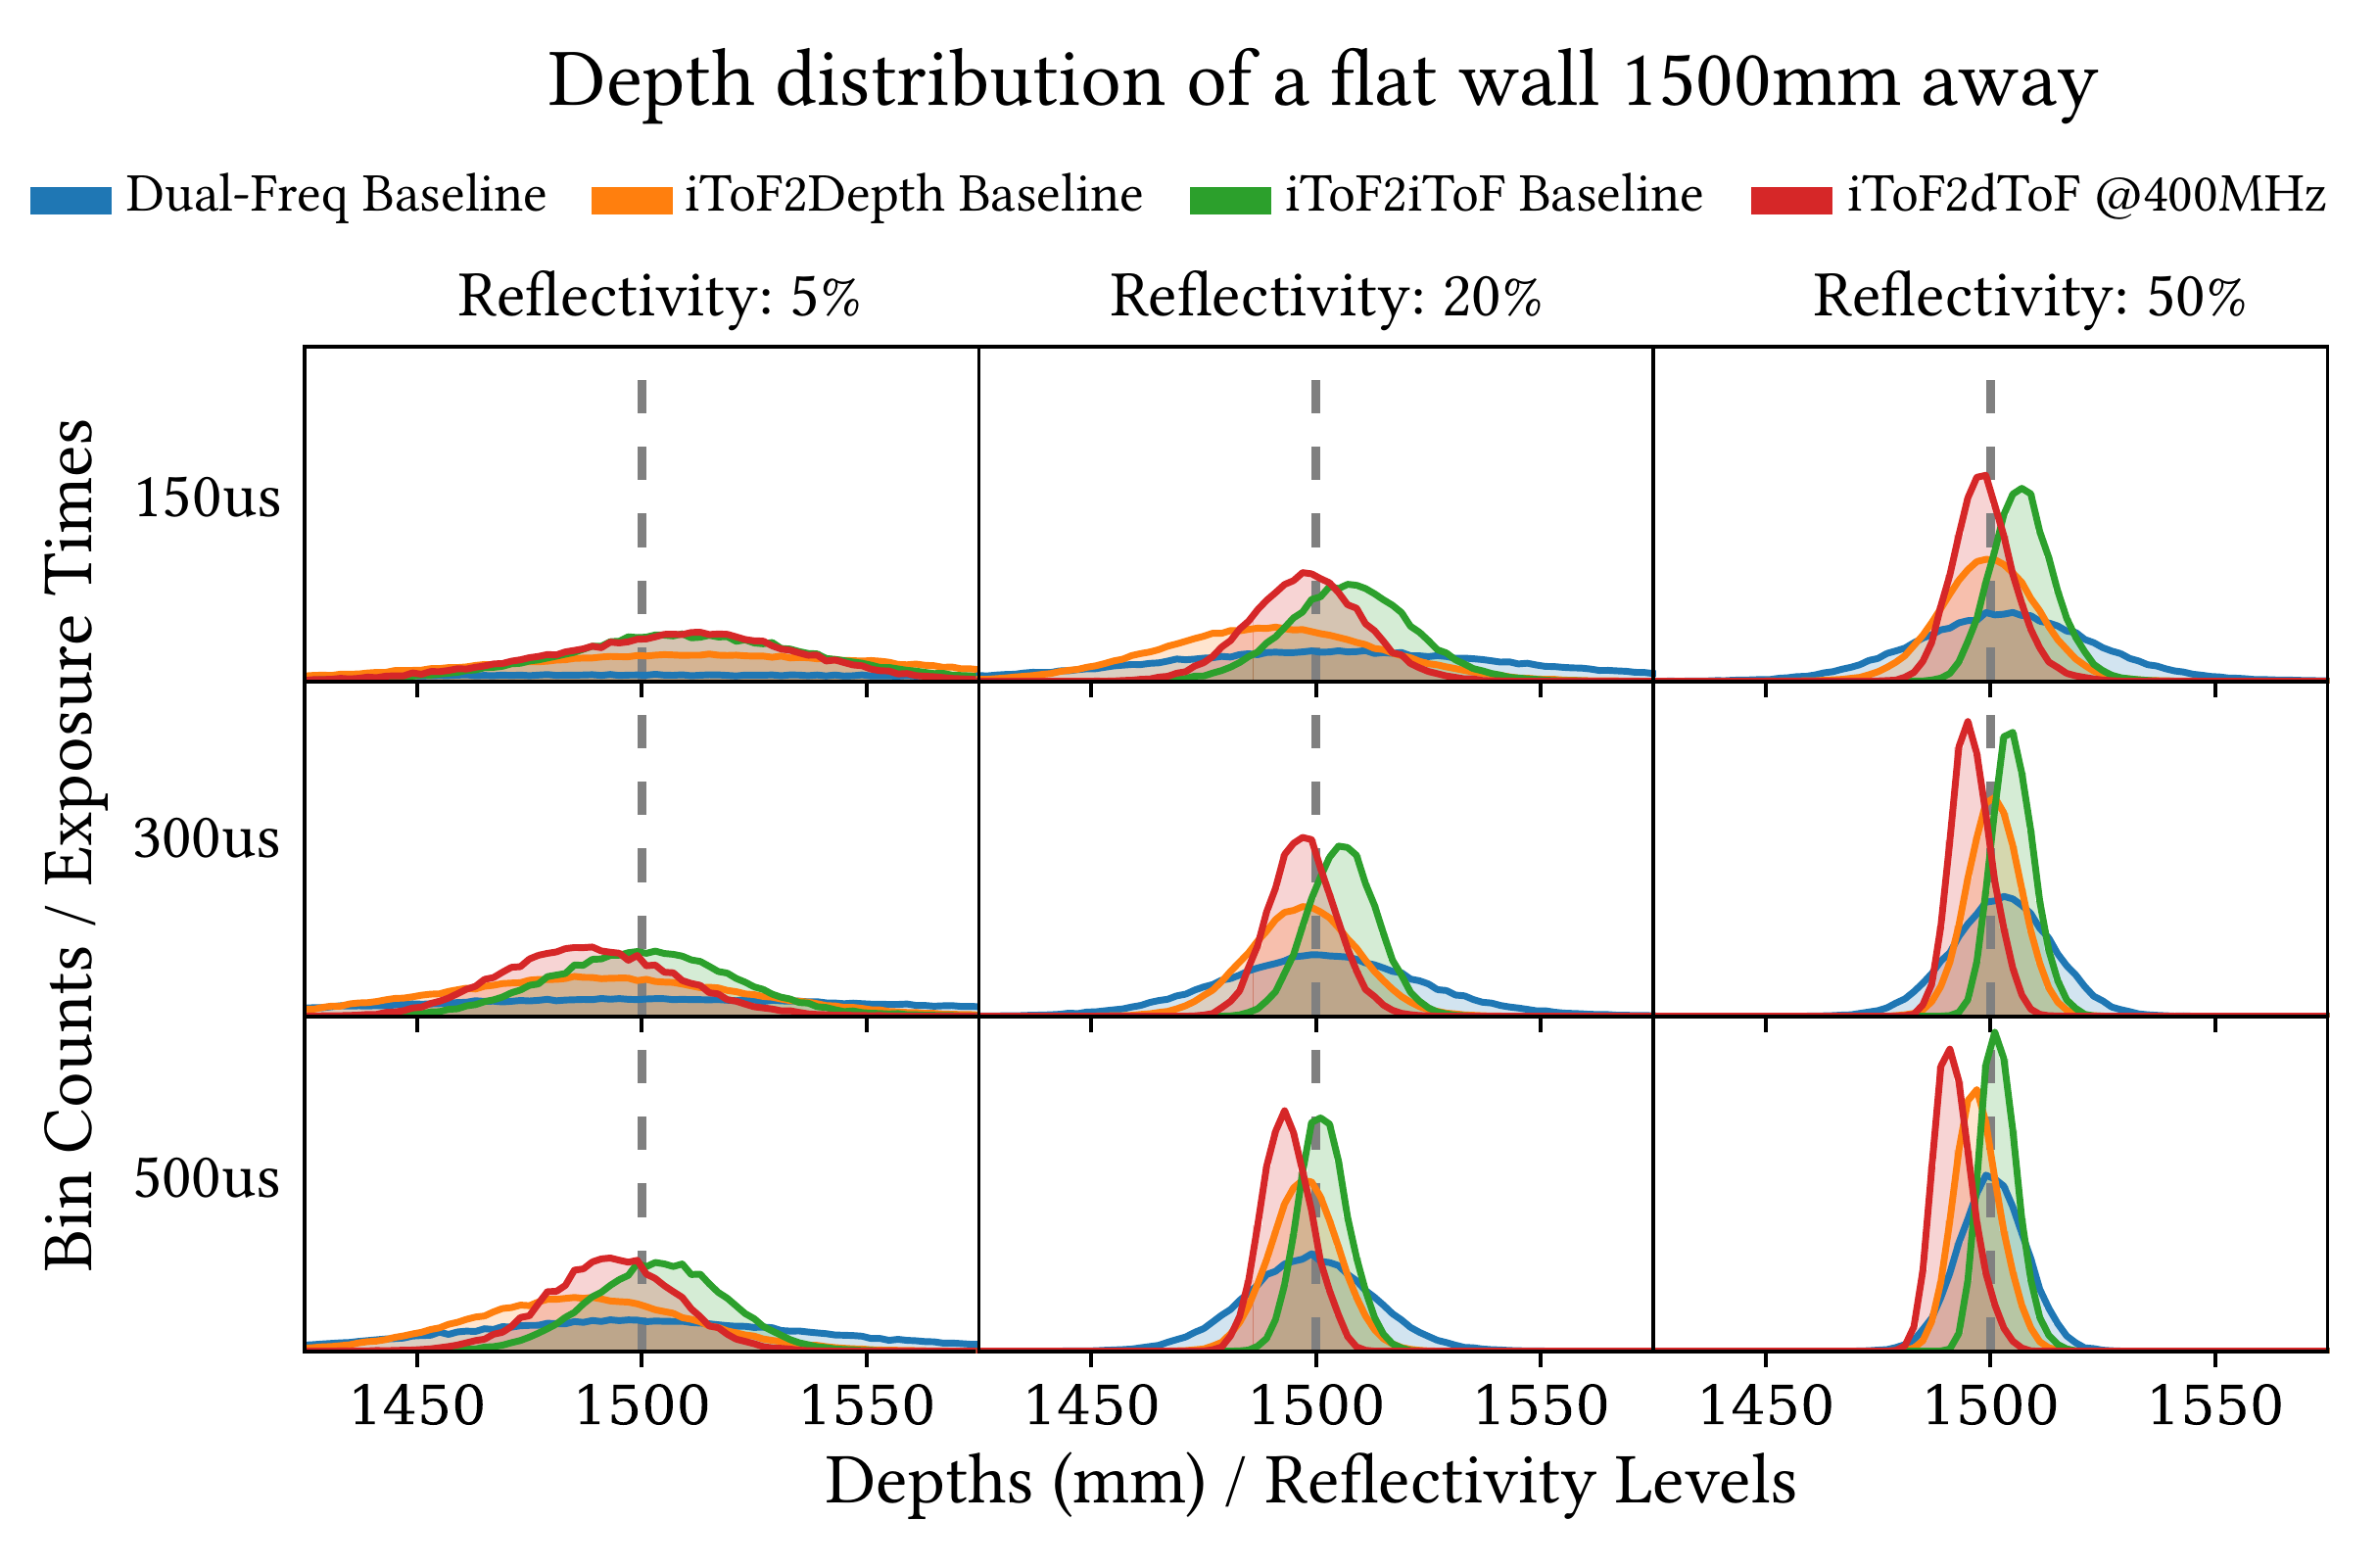}
    \includegraphics[width=0.48\textwidth]{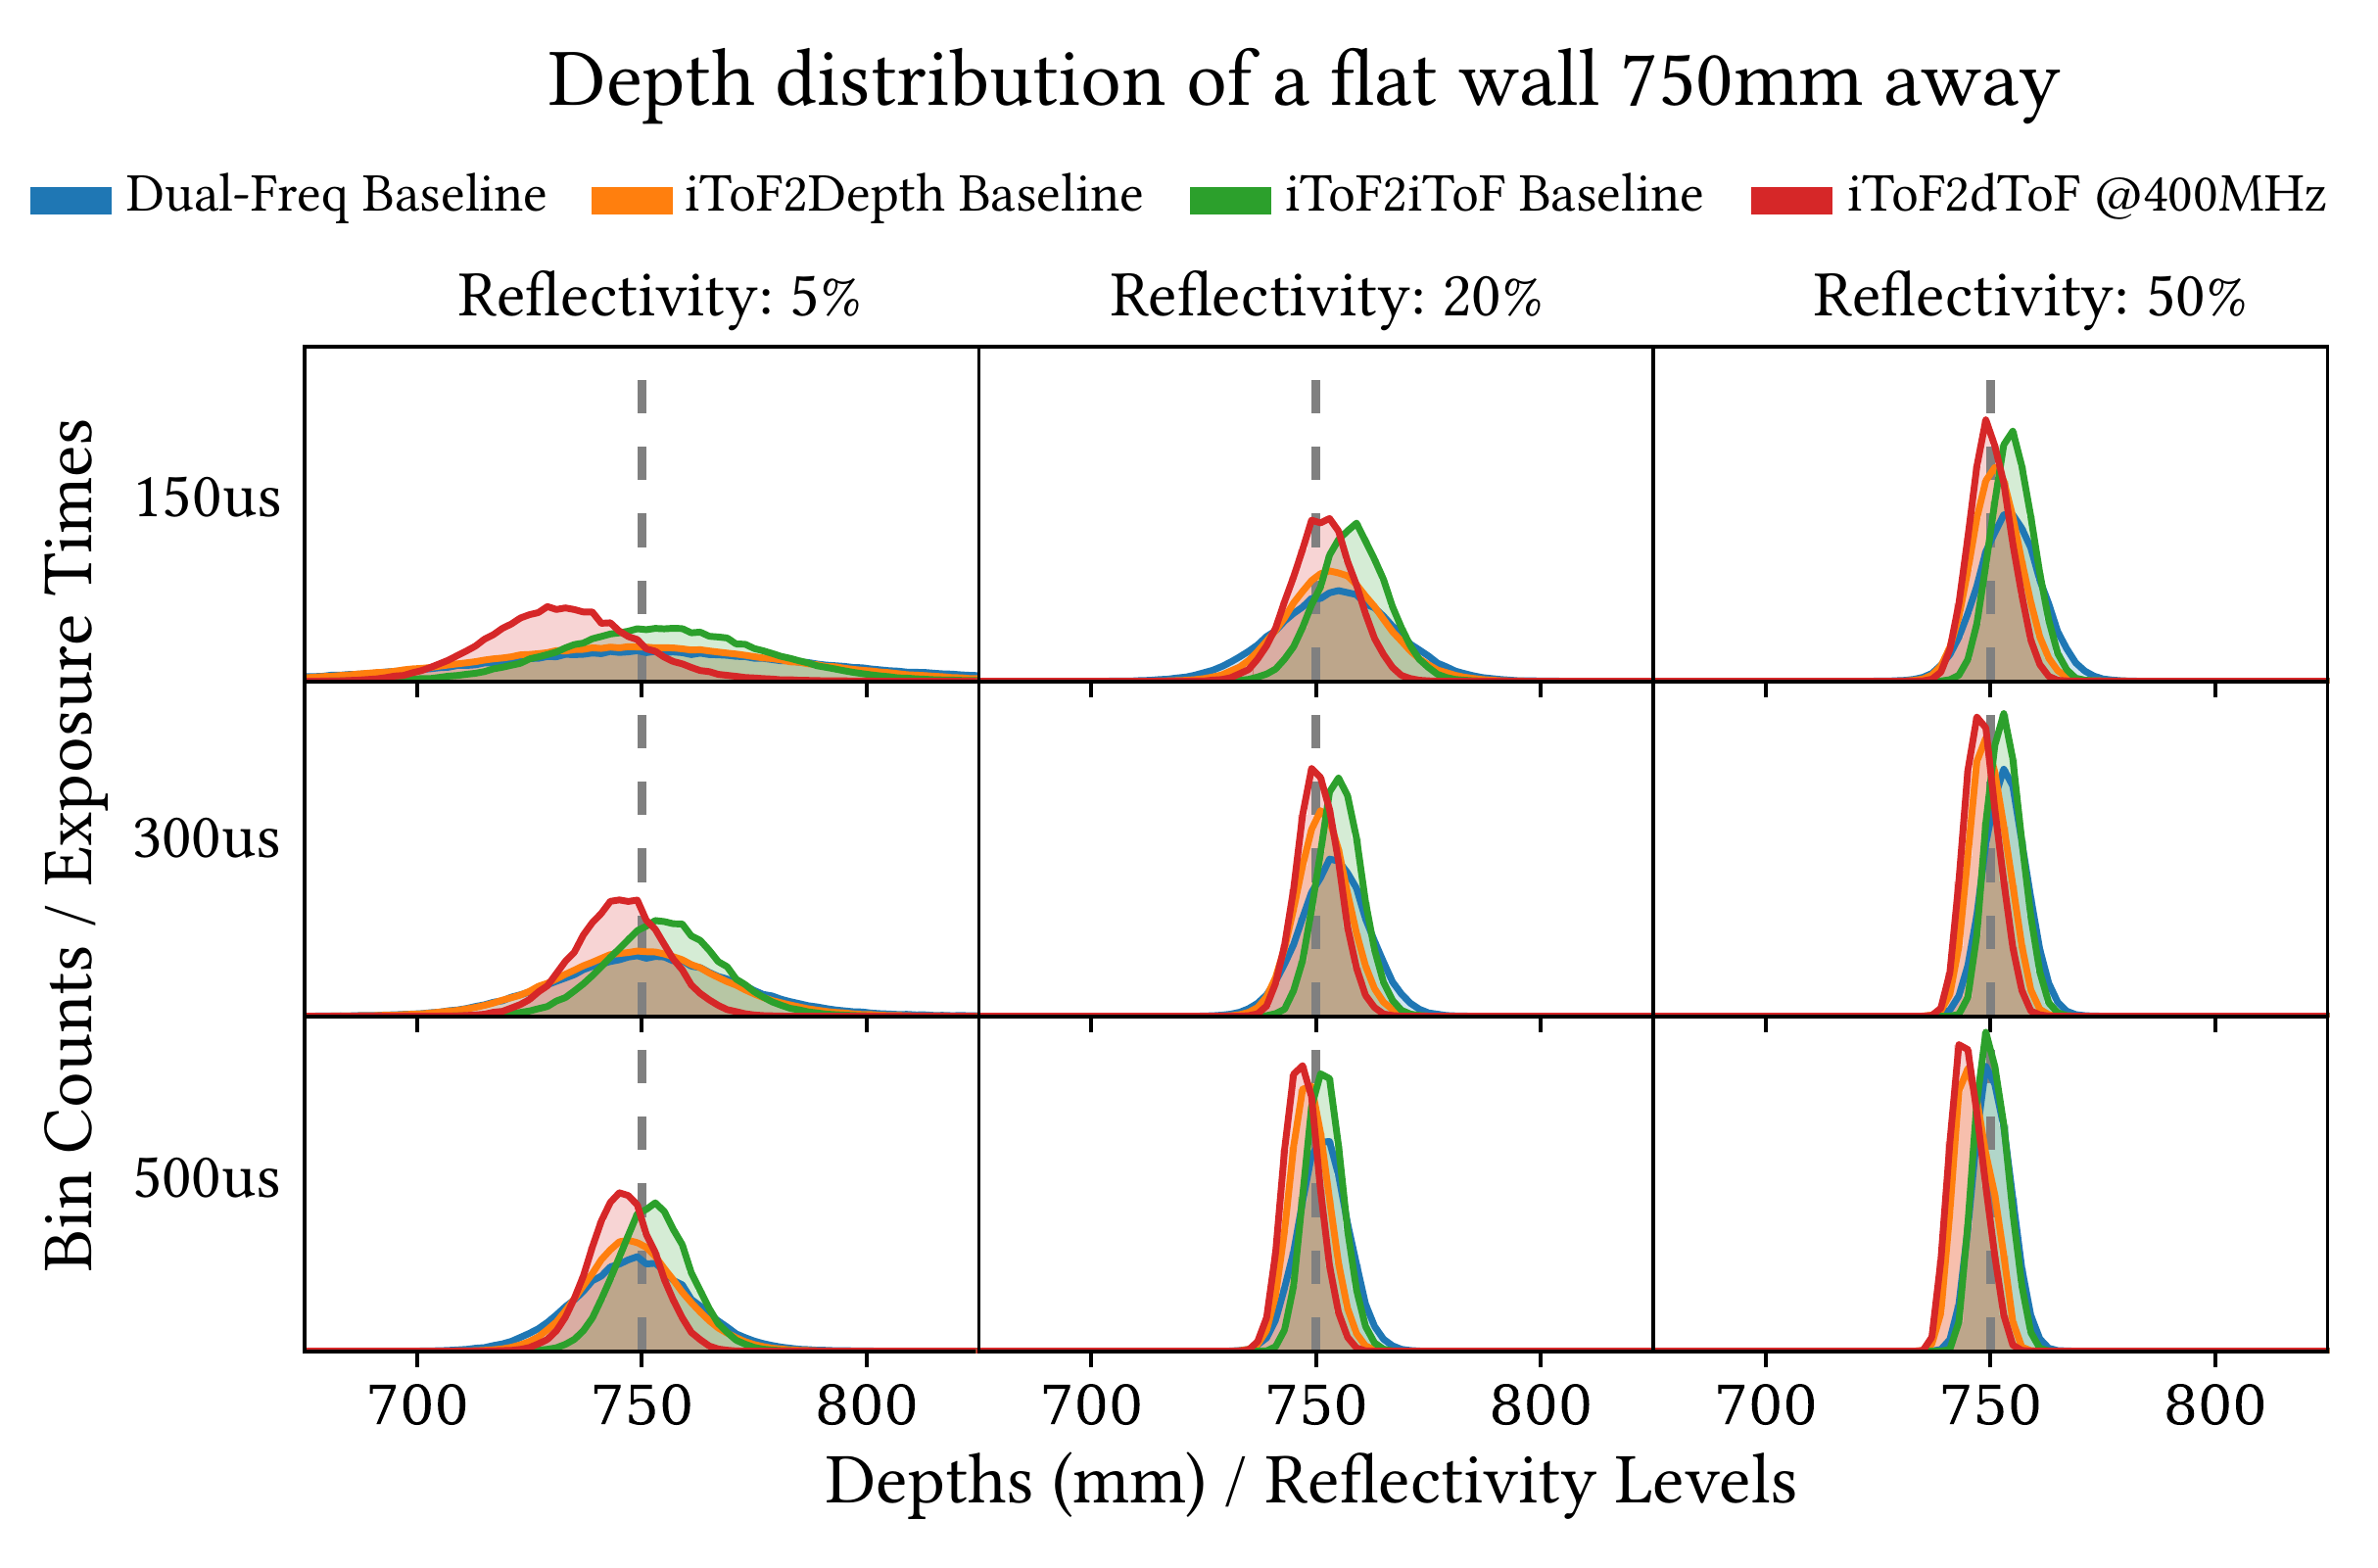}
    \includegraphics[width=0.48\textwidth]{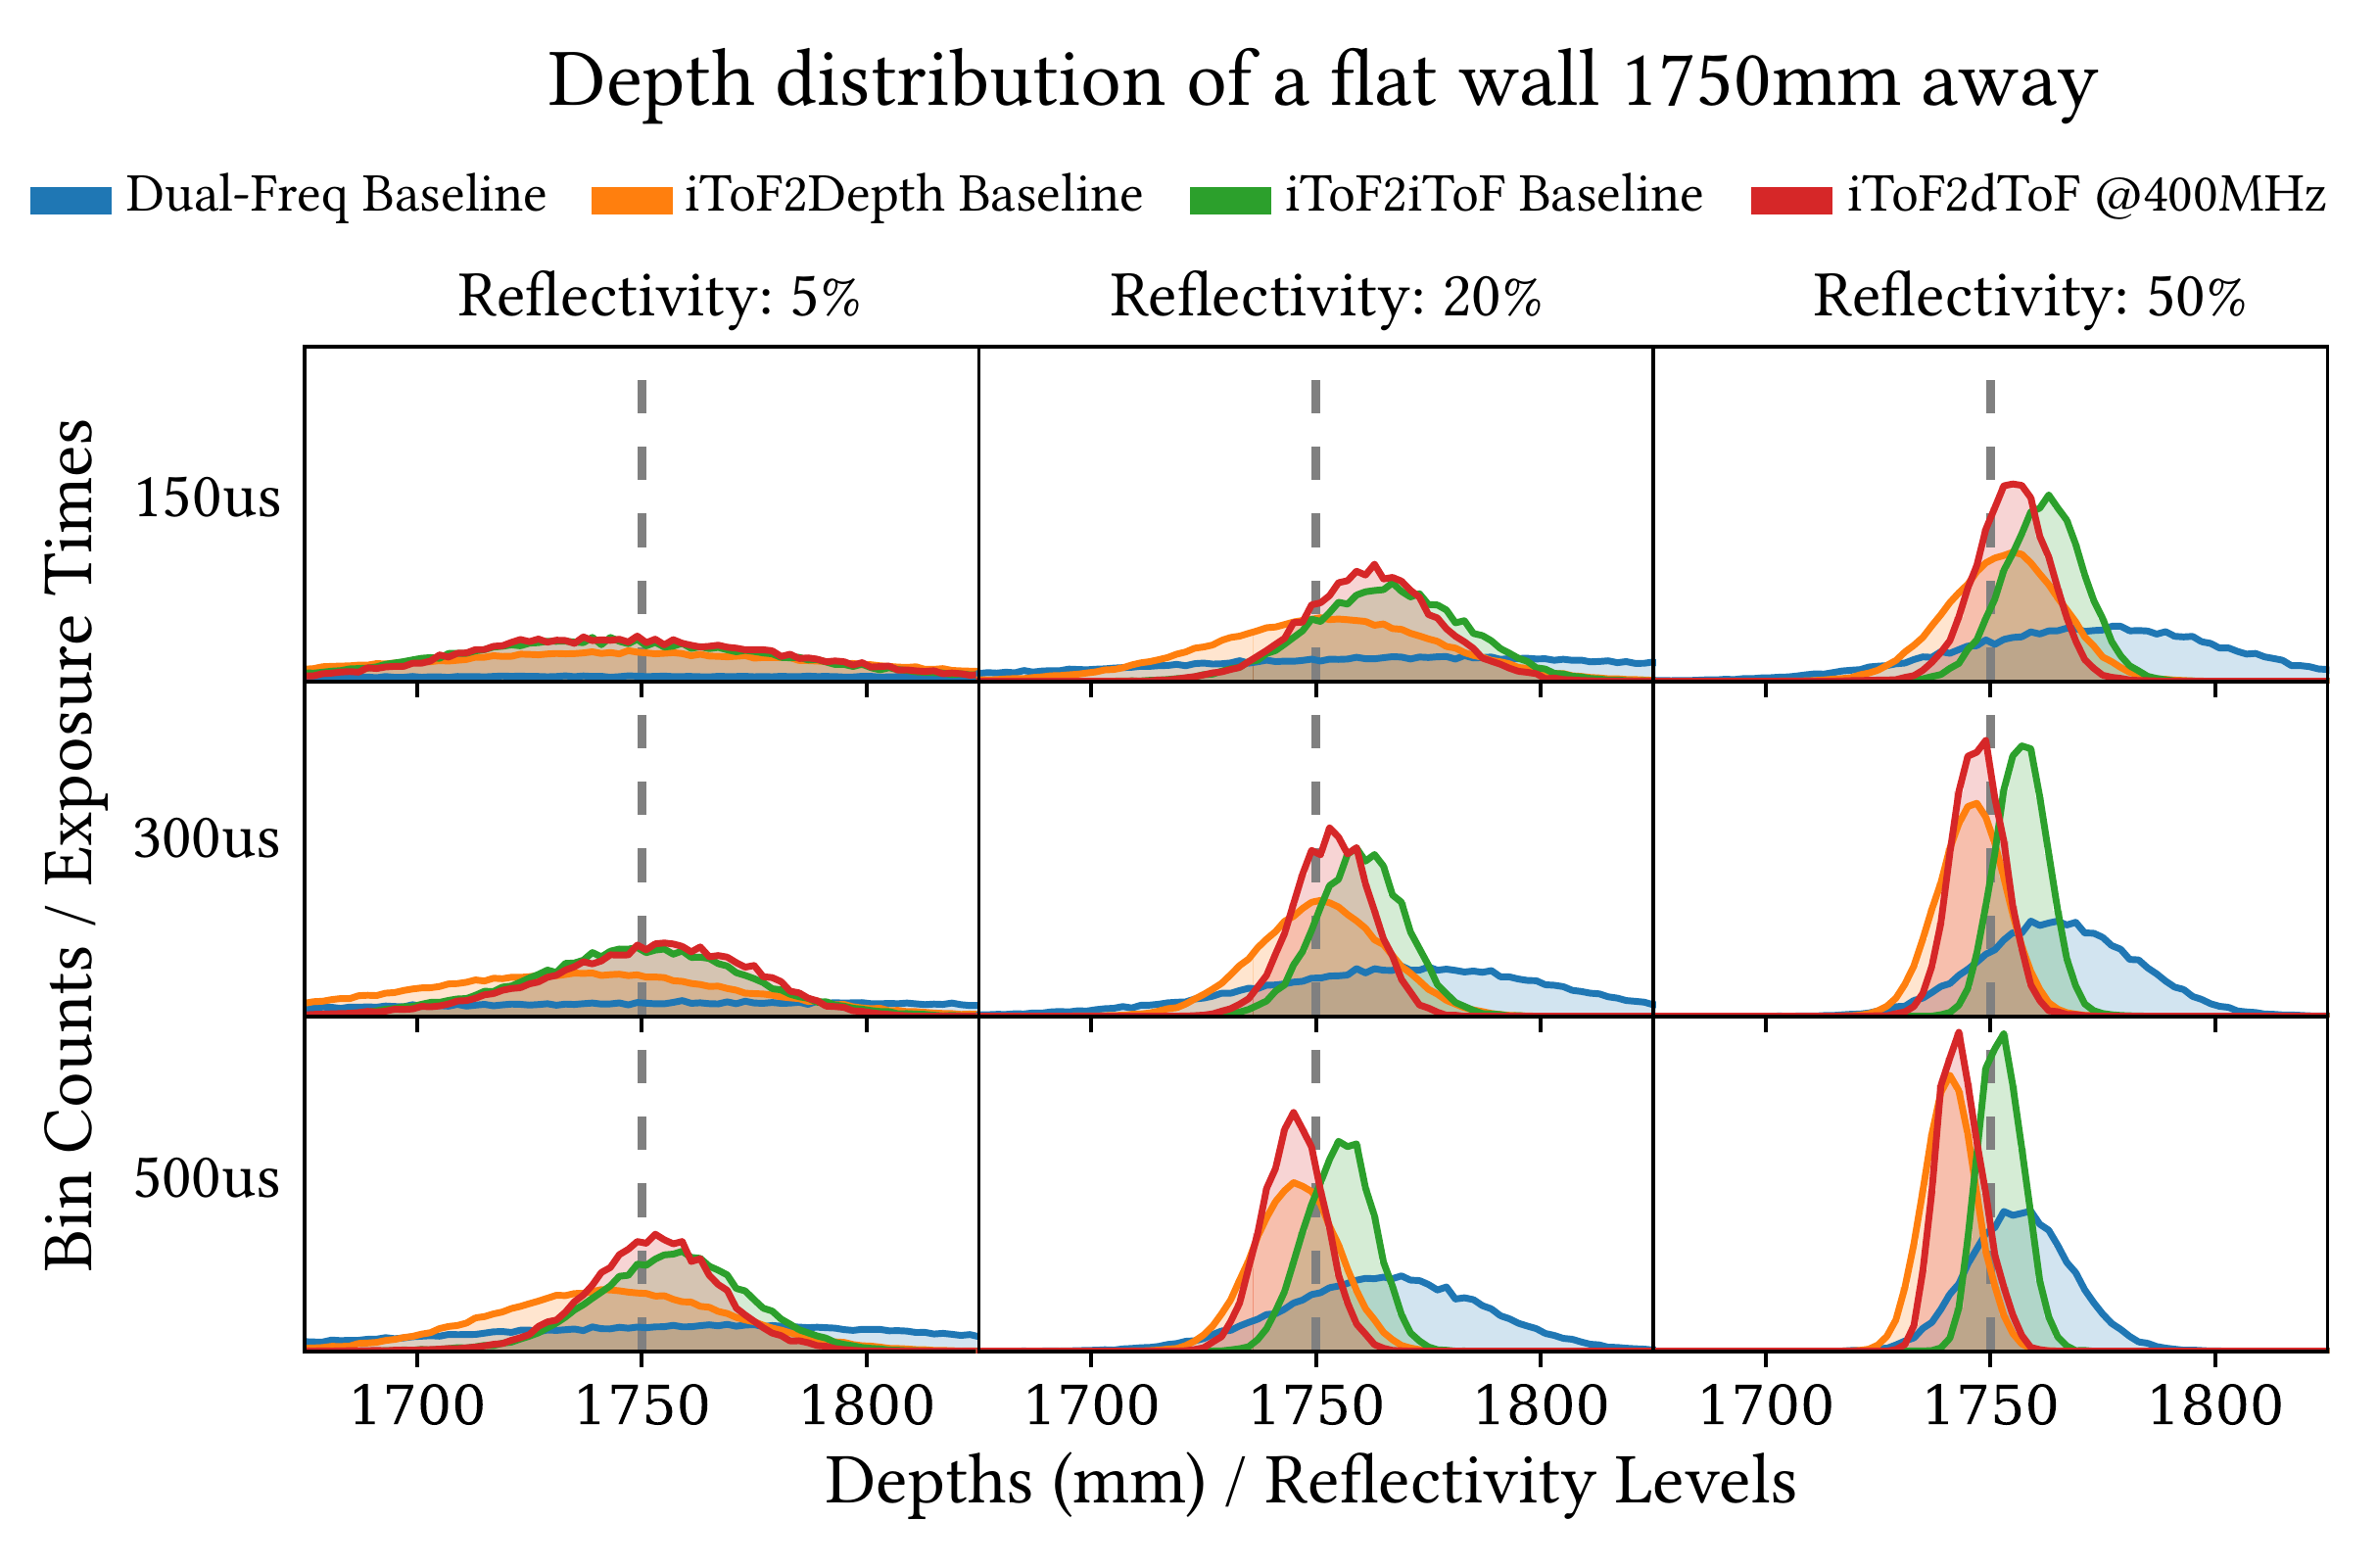}
\caption{\textbf{Wall Depth Histograms}.}
\label{fig:supplement_depth_hist}
\end{figure}
