# Supplementary material for: iToF2dToF: A Robust and Flexible Representation for Data-Driven Time-of-Flight Imaging
Source: arXiv:2103.07087 source file (2021-12-21)
Supplement: Supplementary file 5 [file supplement-2_frequency_analysis.tex]

\clearpage
\section{Frequency Analysis}
\label{sec:supplement-3_frequency_analysis}

Figure \ref{fig:frequency_vs_errors} 

\begin{figure}[H]
\centering
    \includegraphics[width=0.99\textwidth]{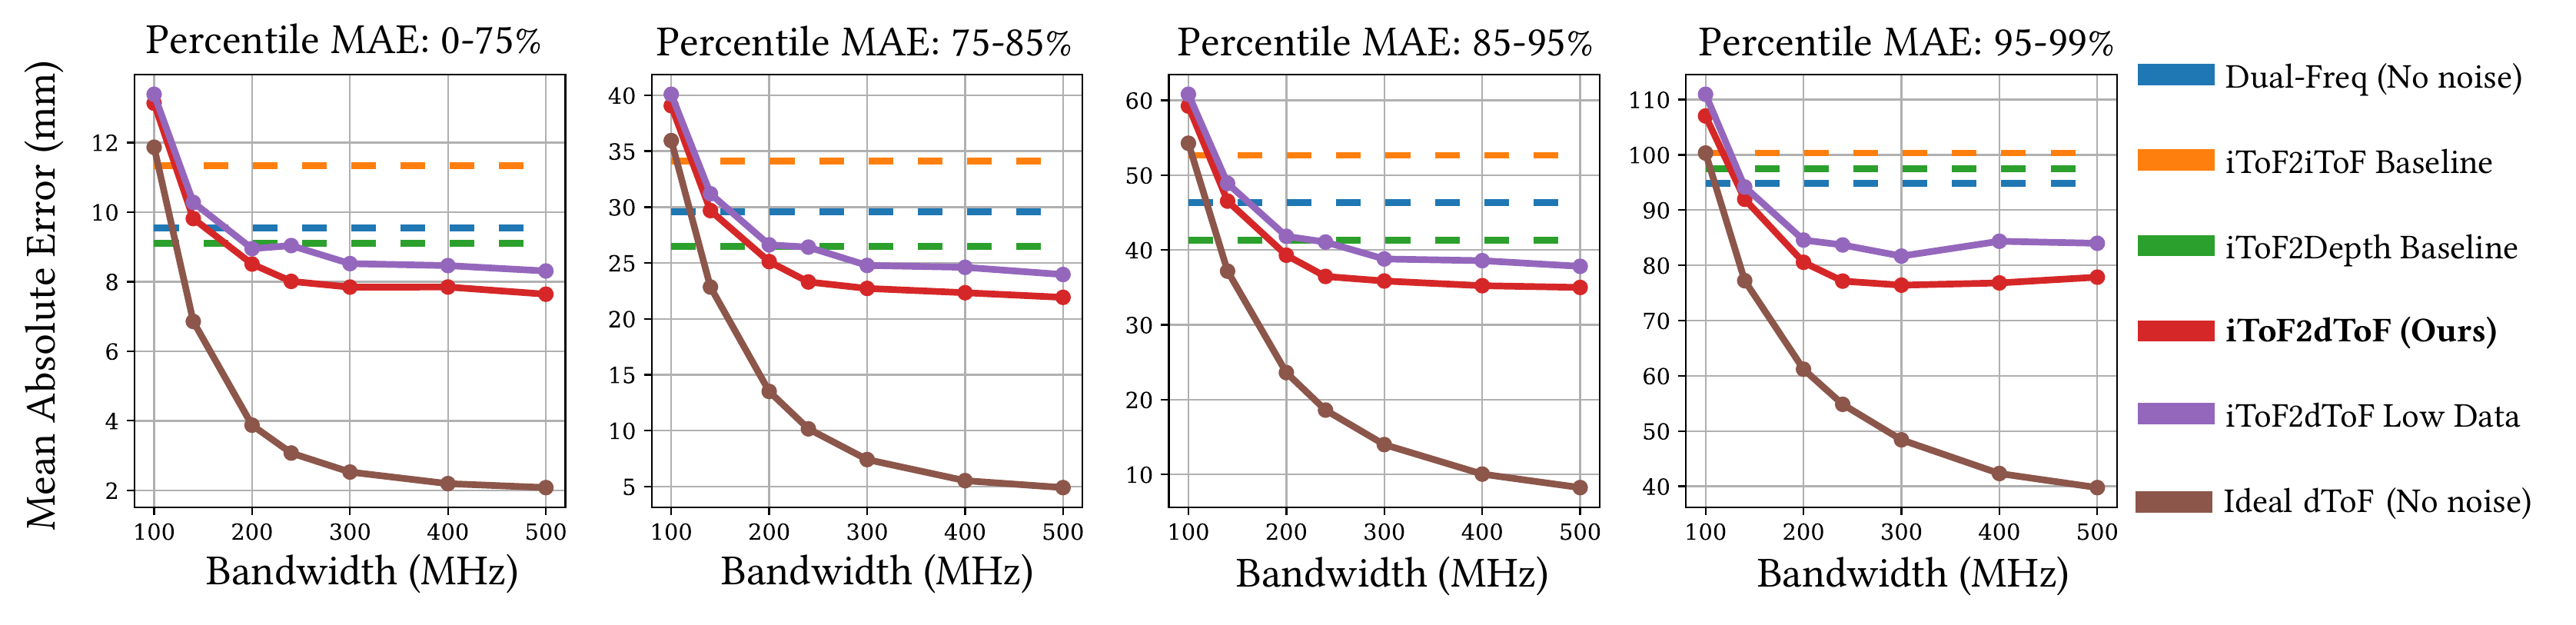}
\caption{\textbf{Frequency vs. Depth Errors}. }
\label{fig:frequency_vs_errors}
\end{figure}
